# Supplementary material for: Non-Shannon inequalities in the entropy vector approach to causal structures
Source: arXiv:1605.02078 ancillary file (2018-03-11)
Supplement: Supplementary file 1 [file SupplementaryInformation.pdf]

# Supplementary Information: Classes of relevant inequalities for causal structures

Mirjam Weilenmann and Roger Colbeck

25th January 2018

In this document we present equivalence classes of inequalities defining outer approximation to the entropy cone of the classical triangle causal structure and a causal structure relevant for the analysis of the principle of information causality, $IC_{\mathrm{R}}^{\mathrm{C}}$, described in the main text.

## 1 Entropy inequalities for the triangle causal structure

In the following we provide the inequalities characterising our outer approximations to the entropy cone of $C_3^{\mathrm{C}}$, taking non-Shannon inequalities into account. We provide these inequalities as tables listing the equivalence classes of inequalities in terms of their coefficients, meaning that each row contains the coefficients $c_1, c_2, \ldots, c_7$ of one representative, $c_1 H(X) + c_2 H(Y) + c_3 H(Z) + c_4 H(XY) + c_5 H(XZ) + c_6 H(YZ) + c_7 H(XYZ) \geq 0$, of a class of inequalities as well as the number of inequalities $n$ in the class. The other inequalities within each class can be obtained by permuting $X$, $Y$ and $Z$.

### Case 1

| $c_1$ | $c_2$ | $c_3$ | $c_4$ | $c_5$ | $c_6$ | $c_7$ | $n$ |
|---|---|---|---|---|---|---|---|
| -157 | -157 | -139 | 155 | 137 | 147 | -125 | 6 |
| -73 | -63 | -51 | 90 | 78 | 73 | -95 | 6 |
| -63 | -58 | -56 | 75 | 73 | 73 | -85 | 6 |
| -99 | -99 | -93 | 90 | 84 | 94 | -70 | 6 |
| -63 | -51 | -45 | 72 | 60 | 56 | -68 | 6 |
| -87 | -87 | -79 | 85 | 72 | 82 | -65 | 6 |
| -51 | -51 | -45 | 54 | 54 | 56 | -56 | 6 |
| -43 | -43 | -36 | 50 | 43 | 48 | -50 | 6 |
| -63 | -63 | -57 | 57 | 57 | 59 | -47 | 6 |
| -39 | -39 | -33 | 42 | 39 | 41 | -41 | 6 |
| -63 | -63 | -61 | 60 | 48 | 58 | -40 | 6 |
| -39 | -33 | -29 | 44 | 36 | 35 | -40 | 6 |
| -29 | -23 | -19 | 36 | 30 | 27 | -37 | 6 |
| -46 | -46 | -42 | 45 | 41 | 41 | -35 | 3 |
| -33 | -32 | -30 | 33 | 35 | 35 | -34 | 6 |
| -25 | -23 | -19 | 30 | 28 | 27 | -33 | 6 |
| -23 | -22 | -20 | 27 | 27 | 27 | -31 | 6 |
| -21 | -19 | -15 | 26 | 23 | 22 | -28 | 6 |
| -19 | -18 | -16 | 23 | 22 | 22 | -26 | 6 |
| -19 | -19 | -16 | 22 | 21 | 22 | -24 | 6 |
| -27 | -27 | -24 | 24 | 24 | 26 | -20 | 6 |
| -15 | -15 | -12 | 18 | 16 | 17 | -19 | 6 |
| -14 | -12 | -10 | 17 | 15 | 14 | -18 | 6 |

| $c_1$ | $c_2$ | $c_3$ | $c_4$ | $c_5$ | $c_6$ | $c_7$ | $n$ |
|---|---|---|---|---|---|---|---|
| -12 | -11 | -11 | 14 | 14 | 14 | -16 | 3 |
| -11 | -8 | -8 | 13 | 14 | 11 | -16 | 6 |
| -23 | -23 | -21 | 20 | 18 | 23 | -15 | 6 |
| -27 | -27 | -27 | 18 | 24 | 26 | -14 | 6 |
| -9 | -9 | -7 | 12 | 11 | 11 | -14 | 3 |
| -21 | -21 | -20 | 20 | 15 | 20 | -13 | 6 |
| -18 | -18 | -18 | 15 | 15 | 17 | -11 | 3 |
| -13 | -13 | -11 | 13 | 12 | 12 | -11 | 3 |
| -11 | -11 | -10 | 12 | 9 | 12 | -10 | 6 |
| -8 | -8 | -7 | 9 | 8 | 9 | -9 | 6 |
| -7 | -5 | -4 | 9 | 7 | 6 | -9 | 6 |
| -5 | -5 | -3 | 8 | 6 | 6 | -9 | 3 |
| -12 | -12 | -12 | 9 | 11 | 11 | -7 | 3 |
| -8 | -8 | -8 | 7 | 7 | 7 | -5 | 1 |
| -7 | -7 | -6 | 6 | 6 | 7 | -5 | 6 |
| -2 | -2 | -2 | 3 | 3 | 3 | -4 | 1 |
| -7 | -7 | -7 | 4 | 6 | 7 | -3 | 6 |
| -4 | -4 | -4 | 3 | 3 | 4 | -2 | 3 |
| -1 | 0 | 0 | 1 | 1 | 0 | -1 | 3 |
| -1 | -1 | -1 | 0 | 1 | 1 | 0 | 3 |
| 0 | 1 | 1 | 0 | 0 | -1 | 0 | 3 |
| 0 | 0 | 0 | -1 | 0 | 0 | 1 | 3 |

## Case 2

| $c_1$ | $c_2$ | $c_3$ | $c_4$ | $c_5$ | $c_6$ | $c_7$ | $n$ |
|---|---|---|---|---|---|---|---|
| -194 | -194 | -164 | 218 | 218 | 223 | -241 | 6 |
| -233 | -233 | -206 | 245 | 218 | 243 | -225 | 6 |
| -248 | -248 | -203 | 245 | 224 | 240 | -213 | 6 |
| -159 | -149 | -138 | 185 | 174 | 179 | -200 | 6 |
| -232 | -232 | -199 | 241 | 184 | 224 | -185 | 6 |
| -111 | -109 | -93 | 130 | 129 | 130 | -148 | 6 |
| -129 | -119 | -113 | 140 | 134 | 139 | -145 | 6 |
| -134 | -134 | -114 | 128 | 138 | 143 | -131 | 6 |
| -109 | -109 | -94 | 121 | 118 | 123 | -129 | 6 |
| -184 | -184 | -169 | 183 | 136 | 176 | -127 | 6 |
| -178 | -178 | -166 | 160 | 148 | 173 | -125 | 6 |
| -157 | -157 | -139 | 155 | 137 | 147 | -125 | 6 |
| -142 | -142 | -124 | 145 | 112 | 137 | -110 | 6 |
| -98 | -98 | -86 | 104 | 104 | 109 | -109 | 6 |
| -98 | -98 | -72 | 110 | 96 | 101 | -107 | 6 |
| -119 | -119 | -98 | 125 | 104 | 114 | -105 | 6 |
| -88 | -88 | -76 | 94 | 97 | 99 | -102 | 6 |
| -168 | -168 | -165 | 163 | 120 | 152 | -99 | 6 |
| -85 | -85 | -70 | 97 | 88 | 93 | -99 | 6 |
| -99 | -99 | -83 | 105 | 89 | 104 | -95 | 6 |
| -100 | -100 | -79 | 109 | 88 | 96 | -93 | 6 |
| -84 | -84 | -67 | 93 | 76 | 88 | -85 | 6 |
| -63 | -58 | -56 | 75 | 73 | 73 | -85 | 6 |
| -75 | -73 | -63 | 76 | 81 | 82 | -82 | 6 |
| -63 | -61 | -54 | 73 | 72 | 73 | -82 | 6 |
| -74 | -74 | -62 | 80 | 74 | 79 | -79 | 6 |
| -122 | -122 | -119 | 110 | 92 | 117 | -75 | 6 |
| -79 | -79 | -61 | 85 | 73 | 75 | -75 | 6 |
| -99 | -99 | -93 | 90 | 84 | 94 | -70 | 6 |
| -74 | -74 | -56 | 74 | 68 | 73 | -67 | 6 |
| -51 | -49 | -42 | 61 | 57 | 58 | -67 | 6 |
| -87 | -87 | -79 | 85 | 72 | 82 | -65 | 6 |
| -74 | -74 | -66 | 68 | 72 | 77 | -65 | 6 |
| -104 | -104 | -103 | 100 | 74 | 94 | -60 | 6 |
| -76 | -76 | -67 | 73 | 64 | 74 | -59 | 6 |
| -64 | -64 | -56 | 58 | 65 | 67 | -58 | 6 |
| -54 | -53 | -48 | 54 | 59 | 59 | -58 | 6 |
| -62 | -62 | -52 | 62 | 58 | 63 | -57 | 6 |
| -51 | -51 | -45 | 54 | 54 | 56 | -56 | 6 |
| -39 | -38 | -33 | 46 | 46 | 46 | -53 | 6 |
| -57 | -57 | -45 | 57 | 53 | 55 | -51 | 6 |
| -88 | -88 | -86 | 85 | 58 | 83 | -50 | 6 |
| -43 | -43 | -36 | 50 | 43 | 48 | -50 | 6 |
| -45 | -43 | -39 | 46 | 48 | 49 | -49 | 6 |
| -63 | -63 | -57 | 57 | 57 | 59 | -47 | 6 |
| -46 | -46 | -35 | 49 | 44 | 46 | -46 | 6 |
| -35 | -35 | -29 | 41 | 40 | 41 | -46 | 6 |
| -39 | -37 | -32 | 43 | 41 | 42 | -45 | 6 |
| -72 | -72 | -69 | 71 | 48 | 68 | -43 | 6 |
| -39 | -39 | -33 | 42 | 39 | 41 | -41 | 6 |
| -63 | -63 | -61 | 60 | 48 | 58 | -40 | 6 |
| -43 | -43 | -40 | 43 | 40 | 45 | -39 | 6 |
| -50 | -50 | -44 | 44 | 44 | 49 | -37 | 6 |
| -30 | -28 | -27 | 34 | 33 | 34 | -37 | 6 |
| -42 | -41 | -38 | 36 | 43 | 43 | -36 | 6 |
| -40 | -40 | -37 | 37 | 40 | 42 | -36 | 6 |
| -40 | -40 | -31 | 40 | 37 | 39 | -36 | 6 |

| $c_1$ | $c_2$ | $c_3$ | $c_4$ | $c_5$ | $c_6$ | $c_7$ | $n$ |
|---|---|---|---|---|---|---|---|
| -52 | -52 | -49 | 51 | 40 | 48 | -35 | 6 |
| -46 | -46 | -42 | 45 | 41 | 41 | -35 | 3 |
| -33 | -33 | -26 | 36 | 32 | 35 | -35 | 6 |
| -33 | -32 | -30 | 33 | 35 | 35 | -34 | 6 |
| -74 | -74 | -74 | 38 | 68 | 73 | -31 | 6 |
| -27 | -26 | -23 | 28 | 30 | 30 | -31 | 6 |
| -23 | -22 | -20 | 27 | 27 | 27 | -31 | 6 |
| -47 | -47 | -47 | 35 | 41 | 45 | -27 | 6 |
| -24 | -22 | -22 | 25 | 25 | 26 | -26 | 3 |
| -19 | -18 | -16 | 23 | 22 | 22 | -26 | 6 |
| -50 | -50 | -50 | 32 | 44 | 49 | -25 | 6 |
| -44 | -44 | -41 | 44 | 26 | 43 | -25 | 6 |
| -34 | -34 | -32 | 28 | 32 | 34 | -25 | 6 |
| -23 | -23 | -19 | 23 | 24 | 25 | -24 | 6 |
| -19 | -19 | -16 | 22 | 21 | 22 | -24 | 6 |
| -41 | -41 | -41 | 29 | 37 | 39 | -23 | 6 |
| -39 | -39 | -37 | 39 | 22 | 40 | -22 | 6 |
| -32 | -32 | -29 | 32 | 23 | 31 | -22 | 6 |
| -28 | -28 | -25 | 25 | 25 | 27 | -21 | 6 |
| -20 | -20 | -14 | 23 | 19 | 19 | -21 | 3 |
| -17 | -17 | -12 | 20 | 17 | 18 | -20 | 6 |
| -17 | -16 | -15 | 18 | 19 | 19 | -20 | 6 |
| -15 | -15 | -11 | 18 | 17 | 17 | -20 | 3 |
| -32 | -32 | -32 | 26 | 26 | 31 | -19 | 3 |
| -27 | -27 | -25 | 27 | 19 | 28 | -19 | 6 |
| -15 | -15 | -12 | 18 | 16 | 17 | -19 | 6 |
| -40 | -40 | -40 | 22 | 37 | 39 | -18 | 6 |
| -20 | -20 | -17 | 21 | 18 | 18 | -17 | 3 |
| -30 | -30 | -29 | 29 | 18 | 29 | -16 | 6 |
| -18 | -18 | -16 | 18 | 16 | 19 | -16 | 6 |
| -12 | -11 | -11 | 14 | 14 | 14 | -16 | 3 |
| -9 | -9 | -4 | 15 | 10 | 10 | -16 | 3 |
| -28 | -28 | -28 | 19 | 25 | 27 | -15 | 6 |
| -23 | -23 | -21 | 20 | 18 | 23 | -15 | 6 |
| -20 | -20 | -17 | 19 | 16 | 20 | -15 | 6 |
| -22 | -22 | -21 | 21 | 16 | 21 | -14 | 6 |
| -9 | -9 | -7 | 12 | 11 | 11 | -14 | 3 |
| -13 | -13 | -11 | 13 | 13 | 14 | -13 | 6 |
| -18 | -18 | -18 | 15 | 15 | 17 | -11 | 3 |
| -15 | -15 | -14 | 16 | 10 | 16 | -11 | 6 |
| -13 | -13 | -11 | 13 | 12 | 12 | -11 | 3 |
| -11 | -11 | -10 | 12 | 9 | 12 | -10 | 6 |
| -11 | -11 | -8 | 11 | 10 | 11 | -10 | 6 |
| -17 | -17 | -17 | 11 | 16 | 16 | -9 | 3 |
| -8 | -8 | -7 | 9 | 8 | 9 | -9 | 6 |
| -5 | -5 | -3 | 8 | 6 | 6 | -9 | 3 |
| -12 | -12 | -12 | 9 | 11 | 11 | -7 | 3 |
| -8 | -8 | -8 | 7 | 7 | 7 | -5 | 1 |
| -7 | -7 | -6 | 6 | 6 | 7 | -5 | 6 |
| -11 | -11 | -11 | 5 | 10 | 11 | -4 | 6 |
| -2 | -2 | -2 | 3 | 3 | 3 | -4 | 1 |
| -7 | -7 | -7 | 4 | 6 | 7 | -3 | 6 |
| -4 | -4 | -4 | 3 | 3 | 4 | -2 | 3 |
| -1 | 0 | 0 | 1 | 1 | 0 | -1 | 3 |
| -1 | -1 | -1 | 0 | 1 | 1 | 0 | 3 |
| 0 | 1 | 1 | 0 | 0 | -1 | 0 | 3 |
| 0 | 0 | 0 | -1 | 0 | 0 | 1 | 3 |

## 2 Non-Shannon outer approximation to the entropy cone of $IC_{\mathrm{R}}^{\mathrm{C}}$

In this section, we provide an outer approximation to the entropy cone of $IC_{\mathrm{R}}^{\mathrm{C}}$ obtained by taking non-Shannon inequalities into account, as specified in the main text. In the following we list the equivalence classes of inequalities in terms of their coefficients, i.e., each row contains the coefficients $c_1, c_2, \ldots, c_{23}$ of one representative,

$$\begin{aligned} c_1H(X_0) + c_2H(X_2) + c_3H(Z) + c_4H(Y_{\mathrm{R}=0}) + c_5H(Y_{\mathrm{R}=1}) + c_6H(X_0X_1) + c_7H(X_0Z) + c_8H(X_0Y_{\mathrm{R}=0}) + c_9H(X_0Y_{\mathrm{R}=1}) \\ + c_{10}H(X_1Z) + c_{11}H(X_1Y_{\mathrm{R}=0}) + c_{12}H(X_1Y_{\mathrm{R}=1}) + c_{13}H(ZY_{\mathrm{R}=0}) + c_{14}H(ZY_{\mathrm{R}=1}) + c_{15}H(X_0X_1Z) + c_{16}H(X_0X_1Y_{\mathrm{R}=0}) \\ + c_{17}H(X_0X_1Y_{\mathrm{R}=1}) + c_{18}H(X_0ZY_{\mathrm{R}=0}) + c_{19}H(X_0ZY_{\mathrm{R}=1}) + c_{20}H(X_1ZY_{\mathrm{R}=0}) + c_{21}H(X_1ZY_{\mathrm{R}=1}) + c_{22}H(X_0X_1ZY_{\mathrm{R}=0}) \\ + c_{23}H(X_0X_1ZY_{\mathrm{R}=1}) \geq 0, \end{aligned}$$

of a class of inequalities as well as the number of inequalities $n$ in the class. The other inequalities in the class can be obtained by permuting $X_0$ and $X_1$ or $Y_{\mathrm{R}=0}$ and $Y_{\mathrm{R}=1}$.

| $c_1$ | $c_2$ | $c_3$ | $c_4$ | $c_5$ | $c_6$ | $c_7$ | $c_8$ | $c_9$ | $c_{10}$ | $c_{11}$ | $c_{12}$ | $c_{13}$ | $c_{14}$ | $c_{15}$ | $c_{16}$ | $c_{17}$ | $c_{18}$ | $c_{19}$ | $c_{20}$ | $c_{21}$ | $c_{22}$ | $c_{23}$ | $n$ |
|---|---|---|---|---|---|---|---|---|---|---|---|---|---|---|---|---|---|---|---|---|---|---|---|
| -9 | -2 | -1 | -6 | -6 | 0 | 0 | 9 | 9 | -3 | 7 | 7 | 5 | -1 | 0 | -9 | 0 | -6 | 6 | 0 | 0 | 15 | -15 | 4 |
| -9 | -1 | -2 | -6 | -6 | 0 | 0 | 9 | 9 | -3 | 5 | -1 | 7 | 7 | 0 | -6 | 6 | -9 | 0 | 0 | 0 | 15 | -15 | 4 |
| -2 | -1 | -9 | -6 | -6 | -3 | 0 | 7 | 7 | 0 | 5 | -1 | 9 | 9 | 0 | 0 | 0 | -9 | 0 | -6 | 6 | 15 | -15 | 4 |
| -3 | -2 | -1 | -2 | -2 | 0 | 0 | 3 | 3 | -1 | 3 | 3 | 3 | -1 | 0 | -3 | 0 | -4 | 4 | 0 | 0 | 7 | -7 | 4 |
| -3 | -1 | -2 | -2 | -2 | 0 | 0 | 3 | 3 | -1 | 3 | -1 | 3 | 3 | 0 | -4 | 4 | -3 | 0 | 0 | 0 | 7 | -7 | 4 |
| -2 | -1 | -3 | -2 | -2 | -1 | 0 | 3 | 3 | 0 | 3 | -1 | 3 | 3 | 0 | 0 | 0 | -3 | 0 | -4 | 4 | 7 | -7 | 4 |
| -4 | -1 | 0 | -3 | -2 | 0 | 0 | 4 | 4 | -1 | 3 | 3 | 2 | -1 | 0 | -4 | 0 | -2 | 2 | 0 | 0 | 6 | -6 | 4 |
| -4 | 0 | -1 | -3 | -2 | 0 | 0 | 4 | 4 | -1 | 2 | -1 | 3 | 3 | 0 | -2 | 2 | -4 | 0 | 0 | 0 | 6 | -6 | 4 |
| -2 | -1 | 9 | -6 | -6 | -12 | 0 | 7 | 7 | 0 | 5 | -1 | 0 | 0 | 0 | 0 | 0 | -9 | 0 | -6 | 6 | 15 | -6 | 4 |
| -1 | 0 | -4 | -3 | -2 | -1 | 0 | 3 | 3 | 0 | 2 | -1 | 4 | 4 | 0 | 0 | 0 | -4 | 0 | -2 | 2 | 6 | -6 | 4 |
| -5 | -4 | -1 | -2 | -4 | 6 | 0 | 3 | 7 | -1 | 3 | 7 | 3 | -1 | 0 | -3 | -8 | -4 | 4 | 0 | 0 | 5 | -5 | 4 |
| -5 | -1 | -4 | -2 | -4 | 0 | 6 | 3 | 7 | -1 | 3 | -1 | 3 | 7 | 0 | -4 | 4 | -3 | -8 | 0 | 0 | 5 | -5 | 4 |
| -4 | -2 | 0 | -3 | -1 | 0 | 0 | 4 | 4 | 1 | 3 | 3 | 2 | -2 | 0 | -4 | 0 | -1 | 1 | -1 | 0 | 5 | -5 | 4 |
| -4 | -2 | 0 | -3 | -1 | 0 | 0 | 4 | 4 | 1 | 3 | 3 | 2 | -2 | 0 | -4 | 0 | 0 | 0 | -2 | 1 | 5 | -5 | 4 |
| -4 | -2 | 0 | -1 | -3 | 0 | 0 | 4 | 4 | 1 | 3 | 3 | -2 | 2 | 0 | -4 | 0 | 0 | 0 | 0 | -1 | 5 | -5 | 4 |
| -4 | -1 | -5 | -2 | -4 | -1 | 6 | 3 | 7 | 0 | 3 | -1 | 3 | 7 | 0 | 0 | 0 | -3 | -8 | -4 | 4 | 5 | -5 | 4 |
| -4 | 0 | -2 | -3 | -1 | 0 | 0 | 4 | 4 | 1 | 2 | -2 | 3 | 3 | 0 | -1 | 1 | -4 | 0 | -1 | 0 | 5 | -5 | 4 |
| -4 | 0 | -2 | -3 | -1 | 0 | 0 | 4 | 4 | 1 | 2 | -2 | 3 | 3 | 0 | 0 | 0 | -4 | 0 | -2 | 1 | 5 | -5 | 4 |
| -4 | 0 | -2 | -1 | -3 | 0 | 0 | 4 | 4 | 1 | -2 | 2 | 3 | 3 | 0 | 0 | 0 | -4 | 0 | 0 | -1 | 5 | -5 | 4 |
| -3 | -1 | 2 | -2 | -2 | -2 | 0 | 3 | 3 | -1 | 3 | -1 | 1 | 1 | 0 | -4 | 4 | -3 | 0 | 0 | 0 | 7 | -5 | 4 |
| -2 | 0 | -4 | -3 | -1 | 1 | 0 | 3 | 3 | 0 | 2 | -2 | 4 | 4 | 0 | -2 | 1 | -4 | 0 | 0 | 0 | 5 | -5 | 4 |
| -2 | 0 | -4 | -3 | -1 | 1 | 0 | 3 | 3 | 0 | 2 | -2 | 4 | 4 | 0 | -1 | 0 | -4 | 0 | -1 | 1 | 5 | -5 | 4 |
| -2 | 0 | -4 | -1 | -3 | 1 | 0 | 3 | 3 | 0 | -2 | 2 | 4 | 4 | 0 | 0 | -1 | -4 | 0 | 0 | 0 | 5 | -5 | 4 |
| -14 | -8 | -4 | -13 | -1 | 9 | 12 | 21 | 7 | 1 | 12 | 6 | 13 | -5 | 0 | -16 | -3 | -16 | 0 | -1 | 0 | 4 | -4 | 4 |
| -14 | -8 | -4 | -10 | -4 | 9 | 12 | 15 | 13 | 1 | 6 | 12 | 13 | -5 | 0 | -7 | -12 | -16 | 0 | -1 | 0 | 4 | -4 | 4 |
| -14 | -8 | -4 | -4 | -10 | 9 | 12 | 13 | 15 | 1 | 12 | 6 | -5 | 13 | 0 | -16 | -3 | 0 | -16 | 0 | -1 | 4 | -4 | 4 |
| -14 | -8 | -4 | -1 | -13 | 9 | 12 | 7 | 21 | 1 | 6 | 12 | -5 | 13 | 0 | -7 | -12 | 0 | -16 | 0 | -1 | 4 | -4 | 4 |
| -14 | -4 | -8 | -13 | -1 | 12 | 9 | 21 | 7 | 1 | 13 | -5 | 12 | 6 | 0 | -16 | 0 | -16 | -3 | -1 | 0 | 4 | -4 | 4 |
| -14 | -4 | -8 | -10 | -4 | 12 | 9 | 15 | 13 | 1 | 13 | -5 | 6 | 12 | 0 | -16 | 0 | -7 | -12 | -1 | 0 | 4 | -4 | 4 |
| -14 | -4 | -8 | -4 | -10 | 12 | 9 | 13 | 15 | 1 | -5 | 13 | 12 | 6 | 0 | 0 | -16 | -16 | -3 | 0 | -1 | 4 | -4 | 4 |
| -14 | -4 | -8 | -1 | -13 | 12 | 9 | 7 | 21 | 1 | -5 | 13 | 6 | 12 | 0 | 0 | -16 | -7 | -12 | 0 | -1 | 4 | -4 | 4 |
| -8 | -4 | -14 | -13 | -1 | 1 | 9 | 12 | 6 | 12 | 13 | -5 | 21 | 7 | 0 | -1 | 0 | -16 | -3 | -16 | 0 | 4 | -4 | 4 |
| -8 | -4 | -14 | -10 | -4 | 1 | 9 | 6 | 12 | 12 | 13 | -5 | 15 | 13 | 0 | -1 | 0 | -7 | -12 | -16 | 0 | 4 | -4 | 4 |
| -8 | -4 | -14 | -4 | -10 | 1 | 9 | 12 | 6 | 12 | -5 | 13 | 13 | 15 | 0 | 0 | -1 | -16 | -3 | 0 | -16 | 4 | -4 | 4 |
| -8 | -4 | -14 | -1 | -13 | 1 | 9 | 6 | 12 | 12 | -5 | 13 | 7 | 21 | 0 | 0 | -1 | -7 | -12 | 0 | -16 | 4 | -4 | 4 |
| -6 | -2 | 12 | -7 | -5 | -9 | 0 | 9 | 9 | 1 | 6 | -4 | -1 | 1 | 0 | -7 | 4 | -12 | 0 | 0 | -1 | 16 | -4 | 4 |
| -5 | -2 | -1 | -4 | -1 | 0 | 3 | 6 | 4 | 1 | 3 | 3 | 4 | -2 | 0 | -4 | 0 | -4 | 0 | -1 | 0 | 4 | -4 | 4 |
| -5 | -2 | -1 | -1 | -4 | 0 | 3 | 4 | 6 | 1 | 3 | 3 | -2 | 4 | 0 | -4 | 0 | 0 | -4 | 0 | -1 | 4 | -4 | 4 |
| -5 | -1 | -2 | -4 | -1 | 3 | 0 | 6 | 4 | 1 | 4 | -2 | 3 | 3 | 0 | -4 | 0 | -4 | 0 | -1 | 0 | 4 | -4 | 4 |
| -5 | -1 | -2 | -1 | -4 | 3 | 0 | 4 | 6 | 1 | -2 | 4 | 3 | 3 | 0 | 0 | -4 | -4 | 0 | 0 | -1 | 4 | -4 | 4 |
| -4 | -2 | 0 | -3 | -1 | 0 | 0 | 4 | 4 | 1 | 3 | 3 | 2 | -2 | 0 | -4 | 0 | 0 | 0 | -1 | 0 | 4 | -4 | 4 |
| -4 | -2 | 0 | -1 | -3 | 0 | 0 | 4 | 4 | 1 | 3 | 3 | -2 | 2 | 0 | -4 | 0 | 0 | 0 | 1 | -2 | 4 | -4 | 4 |
| -4 | -2 | 0 | -1 | -3 | 0 | 0 | 4 | 4 | 1 | 3 | 3 | -2 | 2 | 0 | -4 | 0 | 1 | -1 | 0 | -1 | 4 | -4 | 4 |
| -4 | -1 | -3 | -2 | -4 | -2 | 6 | 3 | 7 | 0 | 3 | -1 | 2 | 6 | 0 | 0 | 0 | -3 | -8 | -4 | 4 | 5 | -4 | 4 |
| -4 | 0 | -2 | -3 | -1 | 0 | 0 | 4 | 4 | 1 | 2 | -2 | 3 | 3 | 0 | 0 | 0 | -4 | 0 | -1 | 0 | 4 | -4 | 4 |
| -4 | 0 | -2 | -1 | -3 | 0 | 0 | 4 | 4 | 1 | -2 | 2 | 3 | 3 | 0 | 0 | 0 | -4 | 0 | 1 | -2 | 4 | -4 | 4 |
| -4 | 0 | -2 | -1 | -3 | 0 | 0 | 4 | 4 | 1 | -2 | 2 | 3 | 3 | 0 | 1 | -1 | -4 | 0 | 0 | -1 | 4 | -4 | 4 |
| -3 | -2 | 0 | -2 | -1 | 0 | 0 | 3 | 3 | 1 | 3 | 2 | 1 | -1 | 0 | -4 | 1 | 0 | 0 | -1 | 0 | 4 | -4 | 4 |

| $c_1$ | $c_2$ | $c_3$ | $c_4$ | $c_5$ | $c_6$ | $c_7$ | $c_8$ | $c_9$ | $c_{10}$ | $c_{11}$ | $c_{12}$ | $c_{13}$ | $c_{14}$ | $c_{15}$ | $c_{16}$ | $c_{17}$ | $c_{18}$ | $c_{19}$ | $c_{20}$ | $c_{21}$ | $c_{22}$ | $c_{23}$ | $n$ |
|---|---|---|---|---|---|---|---|---|---|---|---|---|---|---|---|---|---|---|---|---|---|---|---|
| -3 | -2 | 0 | -1 | -2 | 0 | 0 | 3 | 3 | 1 | 3 | 2 | -1 | 1 | 0 | -4 | 1 | 0 | 0 | 0 | -1 | 4 | -4 | 4 |
| -3 | -2 | 3 | -2 | -1 | -3 | 0 | 3 | 3 | 1 | 3 | -1 | 1 | -1 | 0 | -4 | 4 | -3 | 0 | -1 | 0 | 7 | -4 | 4 |
| -3 | -2 | 3 | -1 | -2 | -3 | 0 | 3 | 3 | 1 | 3 | -1 | -1 | 1 | 0 | -4 | 4 | -3 | 0 | 0 | -1 | 7 | -4 | 4 |
| -3 | 0 | -2 | -2 | -1 | 0 | 0 | 3 | 3 | 1 | 1 | -1 | 3 | 2 | 0 | 0 | 0 | -4 | 1 | -1 | 0 | 4 | -4 | 4 |
| -3 | 0 | -2 | -1 | -2 | 0 | 0 | 3 | 3 | 1 | -1 | 1 | 3 | 2 | 0 | 0 | 0 | -4 | 1 | 0 | -1 | 4 | -4 | 4 |
| -2 | -1 | -5 | -4 | -1 | 1 | 0 | 3 | 3 | 3 | 4 | -2 | 6 | 4 | 0 | -1 | 0 | -4 | 0 | -4 | 0 | 4 | -4 | 4 |
| -2 | -1 | -5 | -1 | -4 | 1 | 0 | 3 | 3 | 3 | -2 | 4 | 4 | 6 | 0 | 0 | -1 | -4 | 0 | 0 | -4 | 4 | -4 | 4 |
| -2 | -1 | 3 | -2 | -2 | -4 | 0 | 3 | 3 | 0 | 3 | -1 | 0 | 0 | 0 | 0 | 0 | -3 | 0 | -4 | 4 | 7 | -4 | 4 |
| -2 | 0 | -4 | -3 | -1 | 1 | 0 | 3 | 3 | 0 | 2 | -2 | 4 | 4 | 0 | -1 | 0 | -4 | 0 | 0 | 0 | 4 | -4 | 4 |
| -2 | 0 | -4 | -1 | -3 | 1 | 0 | 3 | 3 | 0 | -2 | 2 | 4 | 4 | 0 | 0 | -1 | -4 | 0 | 1 | -1 | 4 | -4 | 4 |
| -2 | 0 | -4 | -1 | -3 | 1 | 0 | 3 | 3 | 0 | -2 | 2 | 4 | 4 | 0 | 1 | -2 | -4 | 0 | 0 | 0 | 4 | -4 | 4 |
| -2 | 0 | -3 | -2 | -1 | 1 | 0 | 3 | 2 | 0 | 1 | -1 | 3 | 3 | 0 | -1 | 0 | -4 | 1 | 0 | 0 | 4 | -4 | 4 |
| -2 | 0 | -3 | -1 | -2 | 1 | 0 | 3 | 2 | 0 | -1 | 1 | 3 | 3 | 0 | 0 | -1 | -4 | 1 | 0 | 0 | 4 | -4 | 4 |
| -1 | -1 | 0 | -1 | 0 | 0 | 0 | 1 | 1 | 0 | 1 | 1 | 1 | -1 | 0 | -1 | 0 | -1 | 1 | 0 | 0 | 2 | -2 | 4 |
| -1 | -1 | 0 | 0 | -1 | 0 | 0 | 1 | 1 | 0 | 1 | 1 | -1 | 1 | 0 | -1 | 0 | 0 | 0 | 0 | 0 | 2 | -2 | 2 |
| -1 | 0 | -1 | -1 | 0 | 0 | 0 | 1 | 1 | 0 | 1 | -1 | 1 | 1 | 0 | -1 | 1 | -1 | 0 | 0 | 0 | 2 | -2 | 4 |
| -1 | 0 | -1 | -1 | 0 | 0 | 0 | 1 | 1 | 0 | 1 | -1 | 1 | 1 | 0 | 0 | 0 | -1 | 0 | -1 | 1 | 2 | -2 | 4 |
| -1 | 0 | -1 | 0 | -1 | 0 | 0 | 1 | 1 | 0 | -1 | 1 | 1 | 1 | 0 | 0 | 0 | -1 | 0 | 0 | 0 | 2 | -2 | 4 |
| -1 | 0 | 3 | -2 | -2 | -4 | 0 | 3 | 1 | 0 | 1 | 1 | 0 | 0 | 0 | 0 | 0 | -4 | 2 | -1 | 0 | 5 | -2 | 4 |
| -1 | 0 | 3 | -2 | -2 | -4 | 0 | 3 | 2 | 0 | 1 | 0 | 0 | 0 | 0 | 0 | 0 | -4 | 1 | -1 | 1 | 5 | -2 | 4 |
| -1 | 0 | 4 | -3 | -2 | -5 | 0 | 3 | 3 | 0 | 2 | -1 | 0 | 0 | 0 | 0 | 0 | -4 | 0 | -2 | 2 | 6 | -2 | 4 |
| -4 | -4 | -2 | -5 | 0 | 3 | 3 | 6 | 2 | 3 | 6 | 2 | 6 | -2 | 0 | -5 | -1 | -4 | 0 | -4 | 0 | 1 | -1 | 2 |
| -4 | -4 | -2 | -4 | -1 | 3 | 3 | 4 | 4 | 3 | 4 | 4 | 6 | -2 | 0 | -2 | -4 | -4 | 0 | -4 | 0 | 1 | -1 | 2 |
| -4 | -4 | -2 | -1 | -4 | 3 | 3 | 4 | 4 | 3 | 4 | 4 | -2 | 6 | 0 | -5 | -1 | 0 | -4 | 0 | -4 | 1 | -1 | 2 |
| -4 | -4 | -2 | 0 | -5 | 3 | 3 | 2 | 6 | 3 | 2 | 6 | -2 | 6 | 0 | -2 | -4 | 0 | -4 | 0 | -4 | 1 | -1 | 2 |
| -4 | -2 | -4 | -5 | 0 | 3 | 3 | 6 | 2 | 3 | 6 | -2 | 6 | 2 | 0 | -4 | 0 | -5 | -1 | -4 | 0 | 1 | -1 | 4 |
| -4 | -2 | -4 | -4 | -1 | 3 | 3 | 4 | 4 | 3 | 6 | -2 | 4 | 4 | 0 | -4 | 0 | -2 | -4 | -4 | 0 | 1 | -1 | 4 |
| -4 | -2 | -4 | -1 | -4 | 3 | 3 | 4 | 4 | 3 | -2 | 6 | 4 | 4 | 0 | 0 | -4 | -5 | -1 | 0 | -4 | 1 | -1 | 4 |
| -4 | -2 | -4 | 0 | -5 | 3 | 3 | 2 | 6 | 3 | -2 | 6 | 2 | 6 | 0 | 0 | -4 | -2 | -4 | 0 | -4 | 1 | -1 | 4 |
| -4 | -2 | 0 | -3 | -1 | 0 | 0 | 4 | 4 | 1 | 3 | 3 | 2 | -2 | 0 | 0 | -4 | -1 | 1 | -1 | 0 | 1 | -1 | 4 |
| -4 | -2 | 0 | -3 | -1 | 0 | 0 | 4 | 4 | 1 | 3 | 3 | 2 | -2 | 0 | 0 | -4 | 0 | 0 | -2 | 1 | 1 | -1 | 4 |
| -4 | -2 | 0 | -1 | -3 | 0 | 0 | 4 | 4 | 1 | 3 | 3 | -2 | 2 | 0 | 0 | -4 | 0 | 0 | 0 | -1 | 1 | -1 | 4 |
| -4 | 0 | -2 | -3 | -1 | 0 | 0 | 4 | 4 | 1 | 2 | -2 | 3 | 3 | 0 | -1 | 1 | 0 | -4 | -1 | 0 | 1 | -1 | 4 |
| -4 | 0 | -2 | -3 | -1 | 0 | 0 | 4 | 4 | 1 | 2 | -2 | 3 | 3 | 0 | 0 | 0 | 0 | -4 | -2 | 1 | 1 | -1 | 4 |
| -4 | 0 | -2 | -1 | -3 | 0 | 0 | 4 | 4 | 1 | -2 | 2 | 3 | 3 | 0 | 0 | 0 | 0 | -4 | 0 | -1 | 1 | -1 | 4 |
| -3 | -2 | 3 | -2 | -1 | -3 | 0 | 3 | 3 | 1 | 3 | -1 | 1 | -1 | 0 | -4 | 4 | 0 | -3 | -1 | 0 | 4 | -1 | 4 |
| -2 | -2 | 0 | -2 | 0 | 3 | 0 | 3 | 1 | 0 | 3 | 1 | 1 | -1 | 0 | -4 | -1 | -1 | 1 | 0 | 0 | 1 | -1 | 4 |
| -2 | -2 | 0 | -1 | -1 | 3 | 0 | 1 | 3 | 0 | 1 | 3 | 1 | -1 | 0 | -1 | -4 | -1 | 1 | 0 | 0 | 1 | -1 | 4 |
| -2 | -2 | 0 | -1 | -1 | 3 | 0 | 3 | 1 | 0 | 3 | 1 | -1 | 1 | 0 | -4 | -1 | 0 | 0 | 0 | 0 | 1 | -1 | 2 |
| -2 | -2 | 0 | 0 | -2 | 3 | 0 | 1 | 3 | 0 | 1 | 3 | -1 | 1 | 0 | -1 | -4 | 0 | 0 | 0 | 0 | 1 | -1 | 2 |
| -2 | -2 | 3 | -2 | -3 | -3 | 0 | 3 | 3 | 3 | 2 | 1 | -1 | 3 | 0 | -2 | 1 | -4 | 0 | 0 | -4 | 5 | -1 | 4 |
| -2 | -1 | -1 | -2 | 0 | 0 | 3 | 3 | 1 | 0 | 1 | 1 | 3 | -1 | 0 | -1 | 0 | -4 | 0 | 0 | 0 | 1 | -1 | 4 |
| -2 | -1 | -1 | -2 | 0 | 3 | 0 | 3 | 1 | 0 | 3 | -1 | 1 | 1 | 0 | -4 | 0 | -1 | 0 | 0 | 0 | 1 | -1 | 4 |
| -2 | -1 | -1 | 0 | -2 | 0 | 3 | 1 | 3 | 0 | 1 | 1 | -1 | 3 | 0 | -1 | 0 | 0 | -4 | 0 | 0 | 1 | -1 | 4 |
| -2 | -1 | -1 | 0 | -2 | 3 | 0 | 1 | 3 | 0 | -1 | 3 | 1 | 1 | 0 | 0 | -4 | -1 | 0 | 0 | 0 | 1 | -1 | 4 |
| -2 | -1 | 0 | 0 | -2 | -1 | 3 | 1 | 2 | 0 | 1 | 1 | -1 | 3 | 0 | -1 | 1 | 0 | -4 | -1 | 0 | 2 | -1 | 4 |
| -2 | -1 | 1 | -4 | -1 | -2 | 0 | 3 | 3 | 3 | 4 | -2 | 3 | 1 | 0 | -1 | 0 | -4 | 0 | -4 | 0 | 4 | -1 | 4 |
| -2 | -1 | 1 | -1 | -4 | -2 | 0 | 3 | 3 | 3 | -2 | 4 | 1 | 3 | 0 | 0 | -1 | -4 | 0 | 0 | -4 | 4 | -1 | 4 |
| -2 | 0 | -4 | -3 | -1 | 1 | 0 | 3 | 3 | 0 | 2 | -2 | 4 | 4 | 0 | -2 | 1 | 0 | -4 | 0 | 0 | 1 | -1 | 4 |
| -2 | 0 | -4 | -3 | -1 | 1 | 0 | 3 | 3 | 0 | 2 | -2 | 4 | 4 | 0 | -1 | 0 | 0 | -4 | -1 | 1 | 1 | -1 | 4 |
| -2 | 0 | -4 | -1 | -3 | 1 | 0 | 3 | 3 | 0 | -2 | 2 | 4 | 4 | 0 | 0 | -1 | 0 | -4 | 0 | 0 | 1 | -1 | 4 |
| -2 | 0 | -2 | -2 | 0 | 0 | 3 | 3 | 1 | 0 | 1 | -1 | 3 | 1 | 0 | -1 | 1 | -4 | -1 | 0 | 0 | 1 | -1 | 4 |
| -2 | 0 | -2 | -2 | 0 | 0 | 3 | 3 | 1 | 0 | 1 | -1 | 3 | 1 | 0 | 0 | 0 | -4 | -1 | -1 | 1 | 1 | -1 | 4 |
| -2 | 0 | -2 | -1 | -1 | 0 | 3 | 1 | 3 | 0 | 1 | -1 | 1 | 3 | 0 | -1 | 1 | -1 | -4 | 0 | 0 | 1 | -1 | 4 |
| -2 | 0 | -2 | -1 | -1 | 0 | 3 | 1 | 3 | 0 | 1 | -1 | 1 | 3 | 0 | 0 | 0 | -1 | -4 | -1 | 1 | 1 | -1 | 4 |
| -2 | 0 | -2 | -1 | -1 | 0 | 3 | 3 | 1 | 0 | -1 | 1 | 3 | 1 | 0 | 0 | 0 | -4 | -1 | 0 | 0 | 1 | -1 | 4 |
| -2 | 0 | -2 | 0 | -2 | 0 | 3 | 1 | 3 | 0 | -1 | 1 | 1 | 3 | 0 | 0 | 0 | -1 | -4 | 0 | 0 | 1 | -1 | 4 |
| -2 | 0 | 3 | -2 | -1 | -2 | 0 | 3 | 2 | 0 | 1 | -1 | 0 | 0 | 0 | -1 | 0 | -4 | 1 | 0 | 0 | 4 | -1 | 4 |
| -2 | 0 | 3 | -1 | -2 | -2 | 0 | 3 | 2 | 0 | -1 | 1 | 0 | 0 | 0 | 0 | -1 | -4 | 1 | 0 | 0 | 4 | -1 | 4 |
| -2 | 0 | 4 | -3 | -1 | -3 | 0 | 3 | 3 | 0 | 2 | -2 | 0 | 0 | 0 | -2 | 1 | -4 | 0 | 0 | 0 | 5 | -1 | 4 |
| -2 | 0 | 4 | -3 | -1 | -3 | 0 | 3 | 3 | 0 | 2 | -2 | 0 | 0 | 0 | -1 | 0 | -4 | 0 | -1 | 1 | 5 | -1 | 4 |
| -2 | 0 | 4 | -1 | -3 | -3 | 0 | 3 | 3 | 0 | -2 | 2 | 0 | 0 | 0 | 0 | -1 | -4 | 0 | 0 | 0 | 5 | -1 | 4 |

| $c_1$ | $c_2$ | $c_3$ | $c_4$ | $c_5$ | $c_6$ | $c_7$ | $c_8$ | $c_9$ | $c_{10}$ | $c_{11}$ | $c_{12}$ | $c_{13}$ | $c_{14}$ | $c_{15}$ | $c_{16}$ | $c_{17}$ | $c_{18}$ | $c_{19}$ | $c_{20}$ | $c_{21}$ | $c_{22}$ | $c_{23}$ | $n$ |
|---|---|---|---|---|---|---|---|---|---|---|---|---|---|---|---|---|---|---|---|---|---|---|---|
| -1 | -1 | -2 | -2 | 0 | 0 | 0 | 1 | 1 | 3 | 3 | -1 | 3 | 1 | 0 | 0 | 0 | -1 | 0 | -4 | 0 | 1 | -1 | 4 |
| -1 | -1 | -2 | 0 | -2 | 0 | 0 | 1 | 1 | 3 | -1 | 3 | 1 | 3 | 0 | 0 | 0 | -1 | 0 | 0 | -4 | 1 | -1 | 4 |
| -1 | -1 | 0 | -1 | 0 | 0 | 0 | 1 | 1 | 0 | 1 | 1 | 1 | -1 | 0 | -1 | 0 | 0 | 0 | 0 | 0 | 1 | -1 | 2 |
| -1 | -1 | 0 | -1 | 0 | 0 | 0 | 1 | 1 | 0 | 1 | 1 | 1 | -1 | 0 | 0 | -1 | -1 | 1 | 0 | 0 | 1 | -1 | 4 |
| -1 | -1 | 0 | 0 | -1 | 0 | 0 | 1 | 1 | 0 | 1 | 1 | -1 | 1 | 0 | -1 | 0 | 0 | 0 | 1 | -1 | 1 | -1 | 4 |
| -1 | -1 | 0 | 0 | -1 | 0 | 0 | 1 | 1 | 0 | 1 | 1 | -1 | 1 | 0 | 0 | -1 | 0 | 0 | 0 | 0 | 1 | -1 | 2 |
| -1 | 0 | -1 | -1 | 0 | 0 | 0 | 1 | 1 | 0 | 1 | -1 | 1 | 1 | 0 | -1 | 1 | 0 | -1 | 0 | 0 | 1 | -1 | 4 |
| -1 | 0 | -1 | -1 | 0 | 0 | 0 | 1 | 1 | 0 | 1 | -1 | 1 | 1 | 0 | 0 | 0 | -1 | 0 | 0 | 0 | 1 | -1 | 4 |
| -1 | 0 | -1 | -1 | 0 | 0 | 0 | 1 | 1 | 0 | 1 | -1 | 1 | 1 | 0 | 0 | 0 | 0 | -1 | -1 | 1 | 1 | -1 | 4 |
| -1 | 0 | -1 | 0 | -1 | 0 | 0 | 1 | 1 | 0 | -1 | 1 | 1 | 1 | 0 | 0 | 0 | -1 | 0 | 1 | -1 | 1 | -1 | 4 |
| -1 | 0 | -1 | 0 | -1 | 0 | 0 | 1 | 1 | 0 | -1 | 1 | 1 | 1 | 0 | 0 | 0 | 0 | -1 | 0 | 0 | 1 | -1 | 4 |
| -1 | 0 | -1 | 0 | -1 | 0 | 0 | 1 | 1 | 0 | -1 | 1 | 1 | 1 | 0 | 1 | -1 | -1 | 0 | 0 | 0 | 1 | -1 | 4 |
| -1 | 0 | 1 | -1 | 0 | -1 | 0 | 1 | 1 | 0 | 1 | -1 | 0 | 0 | 0 | -1 | 1 | -1 | 0 | 0 | 0 | 2 | -1 | 4 |
| -1 | 0 | 1 | -1 | 0 | -1 | 0 | 1 | 1 | 0 | 1 | -1 | 0 | 0 | 0 | 0 | 0 | -1 | 0 | -1 | 1 | 2 | -1 | 4 |
| -1 | 0 | 1 | 0 | -1 | -1 | 0 | 1 | 1 | 0 | -1 | 1 | 0 | 0 | 0 | 0 | 0 | -1 | 0 | 0 | 0 | 2 | -1 | 4 |
| 0 | 0 | 0 | 0 | 0 | -1 | 0 | 0 | 0 | 0 | 0 | 0 | 0 | 0 | 1 | 0 | 1 | 0 | 0 | 0 | 0 | 0 | -1 | 2 |
| 0 | 0 | 0 | 0 | 0 | 0 | -1 | 0 | 0 | 0 | 0 | 0 | 0 | 0 | 1 | 0 | 0 | 0 | 1 | 0 | 0 | 0 | -1 | 4 |
| 0 | 0 | 0 | 0 | 0 | 0 | 0 | 0 | -1 | 0 | 0 | 0 | 0 | 0 | 0 | 0 | 1 | 0 | 1 | 0 | 0 | 0 | -1 | 4 |
| 0 | 0 | 0 | 0 | 0 | 0 | 0 | 0 | 0 | 0 | 0 | 0 | 0 | -1 | 0 | 0 | 0 | 0 | 1 | 0 | 1 | 0 | -1 | 2 |
| -14 | -8 | -4 | -13 | -1 | 9 | 12 | 21 | 7 | 1 | 12 | 6 | 13 | -5 | 0 | -16 | -3 | -16 | 0 | -1 | 0 | 0 | 0 | 4 |
| -14 | -8 | -4 | -13 | -1 | 9 | 12 | 21 | 7 | 1 | 12 | 6 | 13 | -5 | 0 | -12 | -7 | -16 | 0 | -1 | 0 | 0 | 0 | 4 |
| -14 | -8 | -4 | -10 | -4 | 9 | 12 | 15 | 13 | 1 | 6 | 12 | 13 | -5 | 0 | -7 | -12 | -16 | 0 | -1 | 0 | 0 | 0 | 4 |
| -14 | -8 | -4 | -10 | -4 | 9 | 12 | 15 | 13 | 1 | 6 | 12 | 13 | -5 | 0 | -3 | -16 | -16 | 0 | -1 | 0 | 0 | 0 | 4 |
| -14 | -4 | -8 | -13 | -1 | 12 | 9 | 21 | 7 | 1 | 13 | -5 | 12 | 6 | 0 | -16 | 0 | -16 | -3 | -1 | 0 | 0 | 0 | 4 |
| -14 | -4 | -8 | -13 | -1 | 12 | 9 | 21 | 7 | 1 | 13 | -5 | 12 | 6 | 0 | -16 | 0 | -12 | -7 | -1 | 0 | 0 | 0 | 4 |
| -14 | -4 | -8 | -10 | -4 | 12 | 9 | 15 | 13 | 1 | 13 | -5 | 6 | 12 | 0 | -16 | 0 | -7 | -12 | -1 | 0 | 0 | 0 | 4 |
| -14 | -4 | -8 | -10 | -4 | 12 | 9 | 15 | 13 | 1 | 13 | -5 | 6 | 12 | 0 | -16 | 0 | -3 | -16 | -1 | 0 | 0 | 0 | 4 |
| -9 | -2 | -1 | -6 | -6 | 0 | 0 | 9 | 9 | -3 | 7 | 7 | -1 | 5 | 0 | 0 | -9 | 6 | -6 | 0 | 0 | 0 | 0 | 4 |
| -9 | -1 | -2 | -6 | -6 | 0 | 0 | 9 | 9 | -3 | -1 | 5 | 7 | 7 | 0 | 6 | -6 | 0 | -9 | 0 | 0 | 0 | 0 | 4 |
| -8 | -4 | -14 | -13 | -1 | 1 | 9 | 12 | 6 | 12 | 13 | -5 | 21 | 7 | 0 | -1 | 0 | -16 | -3 | -16 | 0 | 0 | 0 | 4 |
| -8 | -4 | -14 | -13 | -1 | 1 | 9 | 12 | 6 | 12 | 13 | -5 | 21 | 7 | 0 | -1 | 0 | -12 | -7 | -16 | 0 | 0 | 0 | 4 |
| -8 | -4 | -14 | -10 | -4 | 1 | 9 | 6 | 12 | 12 | 13 | -5 | 15 | 13 | 0 | -1 | 0 | -7 | -12 | -16 | 0 | 0 | 0 | 4 |
| -8 | -4 | -14 | -10 | -4 | 1 | 9 | 6 | 12 | 12 | 13 | -5 | 15 | 13 | 0 | -1 | 0 | -3 | -16 | -16 | 0 | 0 | 0 | 4 |
| -6 | -2 | 12 | -7 | -5 | -9 | 0 | 9 | 9 | 1 | 6 | -4 | -1 | 1 | 0 | -7 | 4 | -12 | 0 | 0 | -1 | 12 | 0 | 4 |
| -6 | -2 | 12 | -4 | -8 | -9 | 0 | 9 | 9 | 1 | -4 | 6 | -1 | 1 | 0 | 4 | -7 | -12 | 0 | 0 | -1 | 12 | 0 | 4 |
| -5 | -4 | -1 | -4 | -2 | 6 | 0 | 7 | 3 | -1 | 7 | 3 | -1 | 3 | 0 | -8 | -3 | 4 | -4 | 0 | 0 | 0 | 0 | 4 |
| -5 | -2 | -1 | -4 | -1 | 0 | 3 | 6 | 4 | 1 | 3 | 3 | 4 | -2 | 0 | -4 | 0 | -4 | 0 | -1 | 0 | 0 | 0 | 4 |
| -5 | -2 | -1 | -4 | -1 | 0 | 3 | 6 | 4 | 1 | 3 | 3 | 4 | -2 | 0 | 0 | -4 | -4 | 0 | -1 | 0 | 0 | 0 | 4 |
| -5 | -1 | -4 | -4 | -2 | 0 | 6 | 7 | 3 | -1 | -1 | 3 | 7 | 3 | 0 | 4 | -4 | -8 | -3 | 0 | 0 | 0 | 0 | 4 |
| -5 | -1 | -2 | -4 | -1 | 3 | 0 | 6 | 4 | 1 | 4 | -2 | 3 | 3 | 0 | -4 | 0 | -4 | 0 | -1 | 0 | 0 | 0 | 4 |
| -5 | -1 | -2 | -4 | -1 | 3 | 0 | 6 | 4 | 1 | 4 | -2 | 3 | 3 | 0 | -4 | 0 | 0 | -4 | -1 | 0 | 0 | 0 | 4 |
| -4 | -4 | -2 | -5 | 0 | 3 | 3 | 6 | 2 | 3 | 6 | 2 | 6 | -2 | 0 | -5 | -1 | -4 | 0 | -4 | 0 | 0 | 0 | 2 |
| -4 | -4 | -2 | -5 | 0 | 3 | 3 | 6 | 2 | 3 | 6 | 2 | 6 | -2 | 0 | -4 | -2 | -4 | 0 | -4 | 0 | 0 | 0 | 2 |
| -4 | -4 | -2 | -4 | -1 | 3 | 3 | 4 | 4 | 3 | 4 | 4 | 6 | -2 | 0 | -2 | -4 | -4 | 0 | -4 | 0 | 0 | 0 | 2 |
| -4 | -4 | -2 | -4 | -1 | 3 | 3 | 4 | 4 | 3 | 4 | 4 | 6 | -2 | 0 | -1 | -5 | -4 | 0 | -4 | 0 | 0 | 0 | 2 |
| -4 | -2 | -4 | -5 | 0 | 3 | 3 | 6 | 2 | 3 | 6 | -2 | 6 | 2 | 0 | -4 | 0 | -5 | -1 | -4 | 0 | 0 | 0 | 4 |
| -4 | -2 | -4 | -5 | 0 | 3 | 3 | 6 | 2 | 3 | 6 | -2 | 6 | 2 | 0 | -4 | 0 | -4 | -2 | -4 | 0 | 0 | 0 | 4 |
| -4 | -2 | -4 | -4 | -1 | 3 | 3 | 4 | 4 | 3 | 6 | -2 | 4 | 4 | 0 | -4 | 0 | -2 | -4 | -4 | 0 | 0 | 0 | 4 |
| -4 | -2 | -4 | -4 | -1 | 3 | 3 | 4 | 4 | 3 | 6 | -2 | 4 | 4 | 0 | -4 | 0 | -1 | -5 | -4 | 0 | 0 | 0 | 4 |
| -4 | -2 | 0 | -3 | -1 | 0 | 0 | 4 | 4 | 1 | 3 | 3 | 2 | -2 | 0 | -4 | 0 | -1 | 1 | -1 | 0 | 0 | 0 | 4 |
| -4 | -2 | 0 | -3 | -1 | 0 | 0 | 4 | 4 | 1 | 3 | 3 | 2 | -2 | 0 | -4 | 0 | 0 | 0 | -2 | 1 | 0 | 0 | 4 |
| -4 | -2 | 0 | -3 | -1 | 0 | 0 | 4 | 4 | 1 | 3 | 3 | 2 | -2 | 0 | 0 | -4 | 0 | 0 | -1 | 0 | 0 | 0 | 4 |
| -4 | -1 | -5 | -4 | -2 | -1 | 6 | 7 | 3 | 0 | -1 | 3 | 7 | 3 | 0 | 0 | 0 | -8 | -3 | 4 | -4 | 0 | 0 | 4 |
| -4 | -1 | -3 | -2 | -4 | -2 | 6 | 3 | 7 | 0 | 3 | -1 | 2 | 6 | 0 | 0 | 0 | -3 | -8 | -4 | 4 | 1 | 0 | 4 |
| -4 | -1 | 0 | -3 | -2 | 0 | 0 | 4 | 4 | -1 | 3 | 3 | 2 | -1 | 0 | -4 | 0 | -2 | 2 | 0 | 0 | 0 | 0 | 4 |
| -4 | 0 | -2 | -3 | -1 | 0 | 0 | 4 | 4 | 1 | 2 | -2 | 3 | 3 | 0 | -1 | 1 | -4 | 0 | -1 | 0 | 0 | 0 | 4 |
| -4 | 0 | -2 | -3 | -1 | 0 | 0 | 4 | 4 | 1 | 2 | -2 | 3 | 3 | 0 | 0 | 0 | -4 | 0 | -2 | 1 | 0 | 0 | 4 |
| -4 | 0 | -2 | -3 | -1 | 0 | 0 | 4 | 4 | 1 | 2 | -2 | 3 | 3 | 0 | 0 | 0 | 0 | -4 | -1 | 0 | 0 | 0 | 4 |
| -4 | 0 | -1 | -3 | -2 | 0 | 0 | 4 | 4 | -1 | 2 | -1 | 3 | 3 | 0 | -2 | 2 | -4 | 0 | 0 | 0 | 0 | 0 | 4 |
| -3 | -2 | -1 | -2 | -2 | 0 | 0 | 3 | 3 | -1 | 3 | 3 | -1 | 3 | 0 | 0 | -3 | 4 | -4 | 0 | 0 | 0 | 0 | 4 |
| -3 | -2 | 0 | -2 | -1 | 0 | 0 | 3 | 3 | 1 | 2 | 3 | 1 | -1 | 0 | 1 | -4 | 0 | 0 | -1 | 0 | 0 | 0 | 4 |
| -3 | -2 | 0 | -2 | -1 | 0 | 0 | 3 | 3 | 1 | 3 | 2 | 1 | -1 | 0 | -4 | 1 | 0 | 0 | -1 | 0 | 0 | 0 | 4 |

| $c_1$ | $c_2$ | $c_3$ | $c_4$ | $c_5$ | $c_6$ | $c_7$ | $c_8$ | $c_9$ | $c_{10}$ | $c_{11}$ | $c_{12}$ | $c_{13}$ | $c_{14}$ | $c_{15}$ | $c_{16}$ | $c_{17}$ | $c_{18}$ | $c_{19}$ | $c_{20}$ | $c_{21}$ | $c_{22}$ | $c_{23}$ | $n$ |
|---|---|---|---|---|---|---|---|---|---|---|---|---|---|---|---|---|---|---|---|---|---|---|---|
| -3 | -2 | 3 | -2 | -1 | -3 | 0 | 3 | 3 | 1 | 3 | -1 | 1 | -1 | 0 | -4 | 4 | -3 | 0 | -1 | 0 | 3 | 0 | 4 |
| -3 | -2 | 3 | -1 | -2 | -3 | 0 | 3 | 3 | 1 | -1 | 3 | -1 | 1 | 0 | 4 | -4 | -3 | 0 | 0 | -1 | 3 | 0 | 4 |
| -3 | -2 | 3 | -1 | -2 | -3 | 0 | 3 | 3 | 1 | 3 | -1 | -1 | 1 | 0 | -4 | 4 | -3 | 0 | 0 | -1 | 3 | 0 | 4 |
| -3 | -1 | -2 | -2 | -2 | 0 | 0 | 3 | 3 | -1 | -1 | 3 | 3 | 3 | 0 | 4 | -4 | 0 | -3 | 0 | 0 | 0 | 0 | 4 |
| -3 | -1 | 2 | -2 | -2 | -2 | 0 | 3 | 3 | -1 | 3 | -1 | 1 | 1 | 0 | -4 | 4 | -3 | 0 | 0 | 0 | 2 | 0 | 4 |
| -3 | 0 | -2 | -2 | -1 | 0 | 0 | 3 | 3 | 1 | 1 | -1 | 2 | 3 | 0 | 0 | 0 | 1 | -4 | -1 | 0 | 0 | 0 | 4 |
| -3 | 0 | -2 | -2 | -1 | 0 | 0 | 3 | 3 | 1 | 1 | -1 | 3 | 2 | 0 | 0 | 0 | -4 | 1 | -1 | 0 | 0 | 0 | 4 |
| -2 | -2 | -1 | 0 | 0 | 3 | 3 | 0 | 1 | 3 | 0 | 1 | 0 | -1 | -4 | 0 | -1 | 0 | 0 | 0 | 0 | 0 | 0 | 2 |
| -2 | -2 | 0 | -2 | 0 | 3 | 0 | 3 | 1 | 0 | 3 | 1 | 1 | -1 | 0 | -4 | -1 | -1 | 1 | 0 | 0 | 0 | 0 | 4 |
| -2 | -2 | 0 | -2 | 0 | 3 | 0 | 3 | 1 | 0 | 3 | 1 | 1 | -1 | 0 | -4 | -1 | 0 | 0 | 0 | 0 | 0 | 0 | 2 |
| -2 | -2 | 0 | -1 | -1 | 3 | 0 | 1 | 3 | 0 | 1 | 3 | 1 | -1 | 0 | -1 | -4 | -1 | 1 | 0 | 0 | 0 | 0 | 4 |
| -2 | -2 | 0 | -1 | -1 | 3 | 0 | 1 | 3 | 0 | 1 | 3 | 1 | -1 | 0 | -1 | -4 | 0 | 0 | 0 | 0 | 0 | 0 | 2 |
| -2 | -2 | 0 | -1 | 0 | 3 | 1 | 3 | 0 | 1 | 3 | 0 | -1 | 0 | -1 | -4 | 0 | 0 | 0 | 0 | 0 | 0 | 0 | 2 |
| -2 | -2 | 3 | -2 | -3 | -3 | 0 | 3 | 3 | 3 | 2 | 1 | -1 | 3 | 0 | -2 | 1 | -4 | 0 | 0 | -4 | 4 | 0 | 4 |
| -2 | -1 | -9 | -6 | -6 | -3 | 0 | 7 | 7 | 0 | -1 | 5 | 9 | 9 | 0 | 0 | 0 | 0 | -9 | 6 | -6 | 0 | 0 | 4 |
| -2 | -1 | -5 | -4 | -1 | 1 | 0 | 3 | 3 | 3 | 4 | -2 | 6 | 4 | 0 | -1 | 0 | -4 | 0 | -4 | 0 | 0 | 0 | 4 |
| -2 | -1 | -5 | -4 | -1 | 1 | 0 | 3 | 3 | 3 | 4 | -2 | 6 | 4 | 0 | -1 | 0 | 0 | -4 | -4 | 0 | 0 | 0 | 4 |
| -2 | -1 | -3 | -2 | -2 | -1 | 0 | 3 | 3 | 0 | -1 | 3 | 3 | 3 | 0 | 0 | 0 | 0 | -3 | 4 | -4 | 0 | 0 | 4 |
| -2 | -1 | -2 | 0 | 0 | 3 | 3 | 0 | 1 | 3 | 0 | -1 | 0 | 1 | -4 | 0 | 0 | 0 | -1 | 0 | 0 | 0 | 0 | 4 |
| -2 | -1 | -1 | -2 | 0 | 0 | 3 | 3 | 1 | 0 | 1 | 1 | 3 | -1 | 0 | -1 | 0 | -4 | 0 | 0 | 0 | 0 | 0 | 4 |
| -2 | -1 | -1 | -2 | 0 | 0 | 3 | 3 | 1 | 0 | 1 | 1 | 3 | -1 | 0 | 0 | -1 | -4 | 0 | 0 | 0 | 0 | 0 | 4 |
| -2 | -1 | -1 | -2 | 0 | 3 | 0 | 3 | 1 | 0 | 3 | -1 | 1 | 1 | 0 | -4 | 0 | -1 | 0 | 0 | 0 | 0 | 0 | 4 |
| -2 | -1 | -1 | -2 | 0 | 3 | 0 | 3 | 1 | 0 | 3 | -1 | 1 | 1 | 0 | -4 | 0 | 0 | -1 | 0 | 0 | 0 | 0 | 4 |
| -2 | -1 | 0 | -2 | 0 | 3 | 1 | 3 | 0 | -1 | 3 | 0 | 1 | 0 | 0 | -4 | 0 | -1 | 0 | 0 | 0 | 0 | 0 | 4 |
| -2 | -1 | 0 | 0 | -2 | -1 | 3 | 1 | 2 | 0 | 1 | 1 | -1 | 3 | 0 | -1 | 1 | 0 | -4 | -1 | 0 | 1 | 0 | 4 |
| -2 | -1 | 1 | -4 | -1 | -2 | 0 | 3 | 3 | 3 | 4 | -2 | 3 | 1 | 0 | -1 | 0 | -4 | 0 | -4 | 0 | 3 | 0 | 4 |
| -2 | -1 | 1 | -2 | 0 | 2 | 0 | 3 | 1 | 0 | 3 | -1 | 0 | 0 | 0 | -4 | 0 | -1 | 0 | 0 | 0 | 1 | 0 | 4 |
| -2 | -1 | 1 | -1 | -4 | -2 | 0 | 3 | 3 | 3 | -2 | 4 | 1 | 3 | 0 | 0 | -1 | -4 | 0 | 0 | -4 | 3 | 0 | 4 |
| -2 | -1 | 1 | 0 | -2 | 2 | 0 | 1 | 3 | 0 | -1 | 3 | 0 | 0 | 0 | 0 | -4 | -1 | 0 | 0 | 0 | 1 | 0 | 4 |
| -2 | -1 | 3 | -2 | -2 | -4 | 0 | 3 | 3 | 0 | 3 | -1 | 0 | 0 | 0 | 0 | 0 | -3 | 0 | -4 | 4 | 3 | 0 | 4 |
| -2 | -1 | 9 | -6 | -6 | -12 | 0 | 7 | 7 | 0 | 5 | -1 | 0 | 0 | 0 | 0 | 0 | -9 | 0 | -6 | 6 | 9 | 0 | 4 |
| -2 | 0 | -4 | -3 | -1 | 1 | 0 | 3 | 3 | 0 | 2 | -2 | 4 | 4 | 0 | -2 | 1 | -4 | 0 | 0 | 0 | 0 | 0 | 4 |
| -2 | 0 | -4 | -3 | -1 | 1 | 0 | 3 | 3 | 0 | 2 | -2 | 4 | 4 | 0 | -1 | 0 | -4 | 0 | -1 | 1 | 0 | 0 | 4 |
| -2 | 0 | -4 | -3 | -1 | 1 | 0 | 3 | 3 | 0 | 2 | -2 | 4 | 4 | 0 | -1 | 0 | 0 | -4 | 0 | 0 | 0 | 0 | 4 |
| -2 | 0 | -3 | -2 | -1 | 1 | 0 | 2 | 3 | 0 | 1 | -1 | 3 | 3 | 0 | -1 | 0 | 1 | -4 | 0 | 0 | 0 | 0 | 4 |
| -2 | 0 | -3 | -2 | -1 | 1 | 0 | 3 | 2 | 0 | 1 | -1 | 3 | 3 | 0 | -1 | 0 | -4 | 1 | 0 | 0 | 0 | 0 | 4 |
| -2 | 0 | -2 | -2 | 0 | 0 | 3 | 3 | 1 | 0 | 1 | -1 | 3 | 1 | 0 | -1 | 1 | -4 | -1 | 0 | 0 | 0 | 0 | 4 |
| -2 | 0 | -2 | -2 | 0 | 0 | 3 | 3 | 1 | 0 | 1 | -1 | 3 | 1 | 0 | 0 | 0 | -4 | -1 | -1 | 1 | 0 | 0 | 4 |
| -2 | 0 | -2 | -2 | 0 | 0 | 3 | 3 | 1 | 0 | 1 | -1 | 3 | 1 | 0 | 0 | 0 | -4 | -1 | 0 | 0 | 0 | 0 | 4 |
| -2 | 0 | -2 | -1 | -1 | 0 | 3 | 1 | 3 | 0 | 1 | -1 | 1 | 3 | 0 | -1 | 1 | -1 | -4 | 0 | 0 | 0 | 0 | 4 |
| -2 | 0 | -2 | -1 | -1 | 0 | 3 | 1 | 3 | 0 | 1 | -1 | 1 | 3 | 0 | 0 | 0 | -1 | -4 | -1 | 1 | 0 | 0 | 4 |
| -2 | 0 | -2 | -1 | -1 | 0 | 3 | 1 | 3 | 0 | 1 | -1 | 1 | 3 | 0 | 0 | 0 | -1 | -4 | 0 | 0 | 0 | 0 | 4 |
| -2 | 0 | -2 | -1 | 0 | 1 | 3 | 3 | 0 | 1 | -1 | 0 | 3 | 0 | -1 | 0 | 0 | -4 | 0 | 0 | 0 | 0 | 0 | 4 |
| -2 | 0 | -1 | -2 | 0 | 1 | 3 | 3 | 0 | -1 | 1 | 0 | 3 | 0 | 0 | -1 | 0 | -4 | 0 | 0 | 0 | 0 | 0 | 4 |
| -2 | 0 | 3 | -2 | -1 | -2 | 0 | 3 | 2 | 0 | 1 | -1 | 0 | 0 | 0 | -1 | 0 | -4 | 1 | 0 | 0 | 3 | 0 | 4 |
| -2 | 0 | 3 | -1 | -2 | -2 | 0 | 3 | 2 | 0 | -1 | 1 | 0 | 0 | 0 | 0 | -1 | -4 | 1 | 0 | 0 | 3 | 0 | 4 |
| -2 | 0 | 4 | -3 | -1 | -3 | 0 | 3 | 3 | 0 | 2 | -2 | 0 | 0 | 0 | -2 | 1 | -4 | 0 | 0 | 0 | 4 | 0 | 4 |
| -2 | 0 | 4 | -3 | -1 | -3 | 0 | 3 | 3 | 0 | 2 | -2 | 0 | 0 | 0 | -1 | 0 | -4 | 0 | -1 | 1 | 4 | 0 | 4 |
| -2 | 0 | 4 | -3 | -1 | -3 | 0 | 3 | 3 | 0 | 2 | -2 | 0 | 0 | 0 | -1 | 0 | -4 | 0 | 0 | 0 | 4 | 0 | 4 |
| -2 | 0 | 4 | -1 | -3 | -3 | 0 | 3 | 3 | 0 | -2 | 2 | 0 | 0 | 0 | 0 | -1 | -4 | 0 | 0 | 0 | 4 | 0 | 4 |
| -2 | 0 | 4 | -1 | -3 | -3 | 0 | 3 | 3 | 0 | -2 | 2 | 0 | 0 | 0 | 0 | -1 | -4 | 0 | 1 | -1 | 4 | 0 | 4 |
| -2 | 0 | 4 | -1 | -3 | -3 | 0 | 3 | 3 | 0 | -2 | 2 | 0 | 0 | 0 | 1 | -2 | -4 | 0 | 0 | 0 | 4 | 0 | 4 |
| -1 | -1 | -2 | -2 | 0 | 0 | 0 | 1 | 1 | 3 | 3 | -1 | 3 | 1 | 0 | 0 | 0 | -1 | 0 | -4 | 0 | 0 | 0 | 4 |
| -1 | -1 | -2 | -2 | 0 | 0 | 0 | 1 | 1 | 3 | 3 | -1 | 3 | 1 | 0 | 0 | 0 | 0 | -1 | -4 | 0 | 0 | 0 | 4 |
| -1 | -1 | 0 | -1 | 0 | 0 | 0 | 1 | 1 | 0 | 1 | 1 | 1 | -1 | 0 | -1 | 0 | -1 | 1 | 0 | 0 | 0 | 0 | 4 |
| -1 | -1 | 0 | -1 | 0 | 0 | 0 | 1 | 1 | 0 | 1 | 1 | 1 | -1 | 0 | 0 | -1 | 0 | 0 | 0 | 0 | 0 | 0 | 2 |
| -1 | 0 | -4 | -3 | -2 | -1 | 0 | 3 | 3 | 0 | 2 | -1 | 4 | 4 | 0 | 0 | 0 | -4 | 0 | -2 | 2 | 0 | 0 | 4 |
| -1 | 0 | -2 | -2 | 0 | -1 | 3 | 3 | 0 | 1 | 1 | 0 | 3 | 0 | 0 | 0 | 0 | -4 | 0 | -1 | 0 | 0 | 0 | 4 |
| -1 | 0 | -1 | -1 | 0 | 0 | 0 | 1 | 1 | 0 | 1 | -1 | 1 | 1 | 0 | -1 | 1 | -1 | 0 | 0 | 0 | 0 | 0 | 4 |
| -1 | 0 | -1 | -1 | 0 | 0 | 0 | 1 | 1 | 0 | 1 | -1 | 1 | 1 | 0 | 0 | 0 | -1 | 0 | -1 | 1 | 0 | 0 | 4 |
| -1 | 0 | -1 | -1 | 0 | 0 | 0 | 1 | 1 | 0 | 1 | -1 | 1 | 1 | 0 | 0 | 0 | 0 | -1 | 0 | 0 | 0 | 0 | 4 |
| -1 | 0 | 0 | 0 | 0 | 0 | 1 | 0 | 1 | 0 | 0 | 0 | 0 | 0 | 0 | 0 | 0 | 0 | -1 | 0 | 0 | 0 | 0 | 4 |

| $c_1$ | $c_2$ | $c_3$ | $c_4$ | $c_5$ | $c_6$ | $c_7$ | $c_8$ | $c_9$ | $c_{10}$ | $c_{11}$ | $c_{12}$ | $c_{13}$ | $c_{14}$ | $c_{15}$ | $c_{16}$ | $c_{17}$ | $c_{18}$ | $c_{19}$ | $c_{20}$ | $c_{21}$ | $c_{22}$ | $c_{23}$ | $n$ |
|---|---|---|---|---|---|---|---|---|---|---|---|---|---|---|---|---|---|---|---|---|---|---|---|
| -1 | 0 | 0 | 0 | 0 | 1 | 0 | 0 | 1 | 0 | 0 | 0 | 0 | 0 | 0 | 0 | -1 | 0 | 0 | 0 | 0 | 0 | 0 | 4 |
| -1 | 0 | 0 | 0 | 0 | 1 | 1 | 0 | 0 | 0 | 0 | 0 | 0 | 0 | -1 | 0 | 0 | 0 | 0 | 0 | 0 | 0 | 0 | 2 |
| -1 | 0 | 1 | -1 | 0 | -1 | 0 | 1 | 1 | 0 | 1 | -1 | 0 | 0 | 0 | -1 | 1 | -1 | 0 | 0 | 0 | 1 | 0 | 4 |
| -1 | 0 | 1 | -1 | 0 | -1 | 0 | 1 | 1 | 0 | 1 | -1 | 0 | 0 | 0 | -1 | 1 | 0 | -1 | 0 | 0 | 1 | 0 | 4 |
| -1 | 0 | 1 | -1 | 0 | -1 | 0 | 1 | 1 | 0 | 1 | -1 | 0 | 0 | 0 | 0 | 0 | -1 | 0 | -1 | 1 | 1 | 0 | 4 |
| -1 | 0 | 1 | -1 | 0 | -1 | 0 | 1 | 1 | 0 | 1 | -1 | 0 | 0 | 0 | 0 | 0 | -1 | 0 | 0 | 0 | 1 | 0 | 4 |
| -1 | 0 | 1 | -1 | 0 | -1 | 0 | 1 | 1 | 0 | 1 | -1 | 0 | 0 | 0 | 0 | 0 | 0 | -1 | -1 | 1 | 1 | 0 | 4 |
| -1 | 0 | 1 | 0 | -1 | -1 | 0 | 1 | 1 | 0 | -1 | 1 | 0 | 0 | 0 | 0 | 0 | -1 | 0 | 0 | 0 | 1 | 0 | 4 |
| -1 | 0 | 1 | 0 | -1 | -1 | 0 | 1 | 1 | 0 | -1 | 1 | 0 | 0 | 0 | 0 | 0 | -1 | 0 | 1 | -1 | 1 | 0 | 4 |
| -1 | 0 | 1 | 0 | -1 | -1 | 0 | 1 | 1 | 0 | -1 | 1 | 0 | 0 | 0 | 0 | 0 | 0 | -1 | 0 | 0 | 1 | 0 | 4 |
| -1 | 0 | 1 | 0 | -1 | -1 | 0 | 1 | 1 | 0 | -1 | 1 | 0 | 0 | 0 | 1 | -1 | -1 | 0 | 0 | 0 | 1 | 0 | 4 |
| -1 | 0 | 3 | -2 | -2 | -4 | 0 | 3 | 1 | 0 | 1 | 1 | 0 | 0 | 0 | 0 | 0 | -4 | 2 | -1 | 0 | 3 | 0 | 4 |
| -1 | 0 | 3 | -2 | -2 | -4 | 0 | 3 | 2 | 0 | 1 | 0 | 0 | 0 | 0 | 0 | 0 | -4 | 1 | -1 | 1 | 3 | 0 | 4 |
| -1 | 0 | 4 | -3 | -2 | -5 | 0 | 3 | 3 | 0 | 2 | -1 | 0 | 0 | 0 | 0 | 0 | -4 | 0 | -2 | 2 | 4 | 0 | 4 |
| 0 | 0 | -1 | 0 | 0 | 0 | 0 | 0 | 0 | 1 | 0 | 0 | 0 | 1 | 0 | 0 | 0 | 0 | 0 | 0 | -1 | 0 | 0 | 4 |
| 0 | 0 | -1 | 0 | 0 | 0 | 1 | 0 | 0 | 1 | 0 | 0 | 0 | 0 | -1 | 0 | 0 | 0 | 0 | 0 | 0 | 0 | 0 | 1 |
| 0 | 0 | 0 | -1 | 0 | 0 | 0 | 0 | 0 | 0 | 1 | 0 | 1 | 0 | 0 | 0 | 0 | 0 | 0 | -1 | 0 | 0 | 0 | 4 |
| 0 | 0 | 0 | -1 | 0 | 0 | 0 | 1 | 0 | 0 | 1 | 0 | 0 | 0 | 0 | -1 | 0 | 0 | 0 | 0 | 0 | 0 | 0 | 2 |
| 0 | 0 | 0 | 0 | 0 | 0 | 0 | 0 | 0 | 0 | 0 | 0 | 0 | 0 | -1 | 0 | 0 | 0 | 0 | 0 | 0 | 1 | 0 | 2 |
| 0 | 0 | 0 | 0 | 0 | 0 | 0 | 0 | 0 | 0 | 0 | 0 | 0 | 0 | 0 | -1 | 0 | 0 | 0 | 0 | 0 | 1 | 0 | 2 |
| 0 | 0 | 0 | 0 | 0 | 0 | 0 | 0 | 0 | 0 | 0 | 0 | 0 | 0 | 0 | 0 | 0 | -1 | 0 | 0 | 0 | 1 | 0 | 4 |
| 0 | 0 | 1 | 0 | 0 | -1 | 0 | 0 | 0 | 0 | 0 | 0 | -1 | 0 | 0 | 0 | 0 | 0 | 0 | 0 | 0 | 1 | 0 | 2 |
| 0 | 0 | 1 | 0 | 0 | -1 | 0 | 0 | 0 | 0 | 0 | 0 | 0 | -1 | 0 | 0 | 0 | -1 | 1 | 0 | 0 | 1 | 0 | 4 |
| 0 | 0 | 1 | 0 | 1 | 0 | 0 | 0 | 0 | 0 | 0 | 0 | 0 | -1 | 0 | 0 | 0 | 0 | 0 | 0 | 0 | 0 | 0 | 2 |
| 0 | 1 | 0 | 0 | 1 | 0 | 0 | 0 | 0 | 0 | 0 | -1 | 0 | 0 | 0 | 0 | 0 | 0 | 0 | 0 | 0 | 0 | 0 | 4 |
| 0 | 1 | 1 | 0 | 0 | 0 | 0 | 0 | 0 | -1 | 0 | 0 | 0 | 0 | 0 | 0 | 0 | 0 | 0 | 0 | 0 | 0 | 0 | 2 |
| 1 | 1 | 0 | 0 | 0 | -1 | 0 | 0 | 0 | 0 | 0 | 0 | 0 | 0 | 0 | 0 | 0 | 0 | 0 | 0 | 0 | 0 | 0 | 1 |
| -2 | 0 | 4 | -3 | -1 | -3 | 0 | 3 | 3 | 0 | 2 | -2 | 0 | 0 | 0 | -1 | 0 | -4 | 0 | 0 | 0 | 3 | 1 | 4 |
| -2 | 0 | 4 | -1 | -3 | -3 | 0 | 3 | 3 | 0 | -2 | 2 | 0 | 0 | 0 | 0 | -1 | -4 | 0 | 1 | -1 | 3 | 1 | 4 |
| -2 | 0 | 4 | -1 | -3 | -3 | 0 | 3 | 3 | 0 | -2 | 2 | 0 | 0 | 0 | 1 | -2 | -4 | 0 | 0 | 0 | 3 | 1 | 4 |
| -6 | -2 | 12 | -4 | -8 | -9 | 0 | 9 | 9 | 1 | -4 | 6 | -1 | 1 | 0 | 4 | -7 | -12 | 0 | 0 | -1 | 8 | 4 | 4 |

# 3 Inner Approximations

In the following, we present inner approximations to the causal structures mentioned in Section IV of the main text, which are listed as structures 4, 5 and 6 in [1] (see Figure 1). We provide these in terms of one vector on each extremal ray of the corresponding marginal entropy cone and we give strategies for recovering these vectors in each case, proving that our extremal rays define an inner approximation. (Note that the inner approximations to causal structures 1, 2 and 3 have been analysed in the main text).

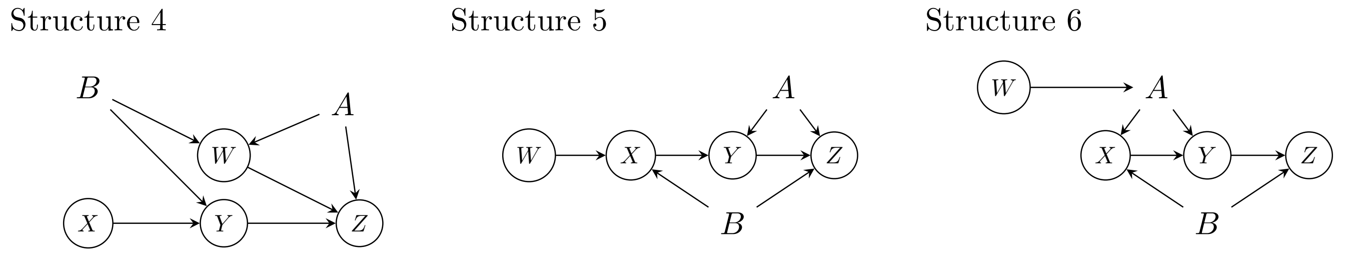


**Figure 1:** Structures 4, 5 and 6 with observed variables $W$, $X$, $Y$ and $Z$ and unobserved $A$ and $B$.

## Causal Structure 4

We provide the vertex description of an inner approximation to the marginal entropy cone of Causal Structure 4 in terms of one vector on each extremal ray, with components ordered as

$$(H(W),\ H(X),\ H(Y),\ H(Z),\ H(WX),\ H(WY),\ H(WZ),\ H(XY),\ H(XZ),\\ H(YZ),\ H(WXY),\ H(WXZ),\ H(WYZ),\ H(XYZ),\ H(WXYZ))\ .$$

| | | | |
|---|---|---|---|
| (1) | 2 2 3 2 4 4 4 4 4 5 5 4 5 5 5 | (21) | 1 1 1 1 2 2 2 2 2 2 3 2 3 3 3 |
| (2) | 2 2 2 1 4 4 3 4 3 3 5 4 5 4 5 | (22) | 1 1 1 1 2 2 2 2 2 2 3 3 3 2 3 |
| (3) | 1 2 2 2 3 3 3 3 3 4 4 3 4 4 4 | (23) | 1 1 1 1 2 2 2 2 2 2 2 2 2 2 2 |
| (4) | 2 1 2 2 3 3 3 3 3 4 4 3 4 4 4 | (24) | 1 1 1 1 2 2 2 2 1 2 3 2 3 2 3 |
| (5) | 2 1 2 2 3 3 4 3 3 3 4 4 4 3 4 | (25) | 1 1 1 1 2 2 1 2 2 2 2 2 2 2 2 |
| (6) | 1 1 2 2 2 3 3 3 3 4 4 4 4 4 4 | (26) | 1 1 1 1 2 2 2 1 2 2 2 2 2 2 2 |
| (7) | 2 1 1 2 3 3 4 2 3 3 4 4 4 4 4 | (27) | 1 1 1 1 2 2 2 2 1 2 2 2 2 2 2 |
| (8) | 2 1 2 1 3 3 3 3 2 3 4 3 4 3 4 | (28) | 1 1 1 1 2 2 2 2 2 1 2 2 2 2 2 |
| (9) | 1 1 1 3 2 2 3 2 3 3 3 3 3 3 3 | (29) | 1 0 1 1 1 2 2 1 1 2 2 2 2 2 2 |
| (10) | 1 1 1 2 2 2 3 2 3 3 3 3 3 3 3 | (30) | 1 1 1 0 2 2 1 2 1 1 2 2 2 2 2 |
| (11) | 1 1 2 1 2 3 2 3 2 3 3 3 3 3 3 | (31) | 0 0 0 1 0 0 1 0 1 1 0 1 1 1 1 |
| (12) | 2 1 1 1 3 3 3 2 2 2 3 3 3 3 3 | (32) | 0 0 1 0 0 1 0 1 0 1 1 0 1 1 1 |
| (13) | 1 1 1 2 2 2 2 2 3 3 3 3 3 3 3 | (33) | 0 1 0 0 1 0 0 1 1 0 1 1 0 1 1 |
| (14) | 1 1 1 2 2 2 3 2 2 3 3 3 3 3 3 | (34) | 1 0 0 0 1 1 1 0 0 0 1 1 1 0 1 |
| (15) | 1 1 1 2 2 2 3 2 3 2 3 3 3 3 3 | (35) | 0 0 1 1 0 1 1 1 1 1 1 1 1 1 1 |
| (16) | 1 1 1 2 2 2 2 2 2 3 3 2 3 3 3 | (36) | 0 1 1 0 1 1 0 1 1 1 1 1 1 1 1 |
| (17) | 1 1 1 2 2 2 3 2 2 2 3 3 3 2 3 | (37) | 1 0 0 1 1 1 1 0 1 1 1 1 1 1 1 |
| (18) | 1 1 1 2 2 2 2 2 2 2 2 2 2 2 2 | (38) | 1 0 1 0 1 1 1 1 0 1 1 1 1 1 1 |
| (19) | 1 1 2 1 2 2 2 2 2 2 2 2 2 2 2 | (39) | 0 1 1 1 1 1 1 1 1 1 1 1 1 1 1 |
| (20) | 1 1 1 1 2 2 2 2 2 2 3 3 3 3 3 | (40) | 1 0 1 1 1 1 1 1 1 1 1 1 1 1 1 |

Below, we list strategies to recover an entropy vector on each of the extremal rays listed above. $C_1$, $C_2$, $C_3$, $C_4$ and $C_5$ are uniformly random bits, $\oplus$ denotes addition modulus 2.

(1) $A = C_1$, $B = (B_1,\ B_2) = (C_2,\ C_3)$, $W = (W_1,\ W_2) = (B_1,\ A \oplus B_2)$, $X = (X_1,\ X_2) = (C_4,\ C_5)$, $Y = (Y_1,\ Y_2,\ Y_3) = (B_1,\ X_1,\ B_2 \oplus X_2)$ and $Z = (W_2 \oplus Y_2, A \oplus W_2 \oplus Y_1 \oplus Y_3)$.

(2) $A = C_1$, $B = (B_1,\ B_2) = (C_2,\ C_3)$, $W = (W_1,\ W_2) = (B_1,\ A \oplus B_2)$, $X = (X_1,\ X_2) = (C_4,\ C_5)$, $Y = (Y_1,\ Y_2) = (B_1 \oplus X_2,\ B_2 \oplus X_1)$ and $Z = (A \oplus W_1 \oplus W_2 \oplus Y_2)$.

(3) $A = C_1$, $B = C_2$, $W = A \oplus B$, $X = (X_1,\ X_2) = (C_3,\ C_4)$, $Y = (Y_1,\ Y_2) = (X_1,\ B \oplus X_2)$ and $Z = (A \oplus W \oplus Y_2,\ W \oplus Y_1)$.

(4) $A = C_1$, $B = (B_1,\ B_2) = (C_2,\ C_3)$, $W = (W_1,\ W_2) = (B_1,\ A \oplus B_2)$, $X = C_4$, $Y = (Y_1,\ Y_2) = (B_1,\ B_2 \oplus X)$ and $Z = (W_2,\ A \oplus W_1 \oplus W_2 \oplus Y_2)$.

(5) $A = C_1$, $B = (B_1,\ B_2) = (C_2,\ C_3)$, $W = (W_1,\ W_2) = (B_1,\ A \oplus B_2)$, $X = C_4$, $Y = (Y_1,\ Y_2) = (B_1,\ B_2 \oplus X)$ and $Z = (Y_2,\ A \oplus W_1 \oplus W_2 \oplus Y_2)$.

(6) $A = C_1$, $B = (B_1,\ B_2) = (C_2,\ C_3)$, $W = A \oplus B_1$, $X = C_4$, $Y = (Y_1,\ Y_2) = (B_1 \oplus X,\ B_2)$ and $Z = (A \oplus Y_2,\ A \oplus W)$.

(7) $A = C_1$, $B = (B_1,\ B_2) = (C_2,\ C_3)$, $W = (W_1,\ W_2) = (A \oplus B_1, B_2)$, $X = C_4$, $Y = B_1 \oplus X$ and $Z = (W_2 \oplus Y,\ A \oplus Y)$.

(8) $A = C_1$, $B = (B_1,\ B_2) = (C_2,\ C_3)$, $W = (W_1,\ W_2) = (A \oplus B_1,\ A \oplus B_2)$, $X = C_4$, $Y = (Y_1,\ Y_2) = (B_1 \oplus X,\ B_2 \oplus X)$ and $Z = A \oplus W_2 \oplus Y_1$.

(9) $A = C_1$, $B = C_2$, $W = A \oplus B$, $X = C_3$, $Y = B \oplus X$ and $Z = (A \oplus W,\ Y,\ A)$.

(10) $A = C_1$, $B = C_2$, $W = A \oplus B$, $X = C_3$, $Y = B \oplus X$ and $Z = (A \oplus Y,\ W \oplus Y)$.

(11) $A = 0$, $B = (B_1,\ B_2) = (C_1,\ C_2)$, $W = B_1$, $X = C_3$, $Y = (Y_1,\ Y_2) = (B_1 \oplus X,\ B_2)$ and $Z = W \oplus Y_2$.

(12) $A = 0$, $B = (B_1,\ B_2) = (C_1,\ C_2)$, $W = (W_1,\ W_2) = (B_1,\ B_2)$, $X = C_3$, $Y = B_1 \oplus X$ and $Z = W_2 \oplus Y$.

(13) $A = C_1$, $B = C_2$, $W = A \oplus B$, $X = C_3$, $Y = B \oplus X$ and $Z = (A \oplus W,\ A)$.

(14) $A = C_1$, $B = C_2$, $W = A \oplus B$, $X = C_3$, $Y = B \oplus X$ and $Z = (W \oplus Y,\ A)$.

(15) $A = C_1$, $B = C_2$, $W = A \oplus B$, $X = C_3$, $Y = B \oplus X$ and $Z = (A \oplus Y,\ A)$.

(16) $A = C_1$, $B = C_2$, $W = A \oplus B$, $X = C_3$, $Y = B \oplus X$ and $Z = (W,\ A \oplus W \oplus Y)$.

(17) $A = C_1$, $B = C_2$, $W = A \oplus B$, $X = C_3$, $Y = B \oplus X$ and $Z = (Y,\ A \oplus W \oplus Y)$.

(18) $A = 0$, $B = C_1$, $W = B$, $X = C_2$, $Y = B \oplus X$ and $Z = (W,\ Y)$.

(19) $A = 0$, $B = C_1$, $W = B$, $X = C_2$, $Y = (Y_1,\ Y_2) = (B, X)$ and $Z = (W \oplus Y_2)$.

(20) $A = C_1$, $B = C_2$, $W = A \oplus B$, $X = C_3$, $Y = B \oplus X$ and $Z = A$.

(21) $A = C_1$, $B = C_2$, $W = A \oplus B$, $X = C_3$, $Y = B \oplus X$ and $Z = A \oplus Y$.

(22) $A = C_1$, $B = C_2$, $W = A \oplus B$, $X = C_3$, $Y = B \oplus X$ and $Z = A \oplus W$.

(23) $A = 0$, $B = (B_1,\ B_2) = (C_1,\ C_2)$, $W = (W_1,\ W_2) = (B_1,\ B_2)$, $X = (X_1,\ X_2) = (C_3,\ C_4)$, $Y = (Y_1,\ Y_2) = (B_2 \oplus X_1 \oplus X_2,\ B_1 \oplus X_1)$ and $Z = (W_1 \oplus W_2 \oplus Y_1,\ W_2 \oplus Y_2)$. [1]

(24) $A = C_1$, $B = C_2$, $W = A \oplus B$, $X = C_3$, $Y = B \oplus X$ and $Z = A \oplus W \oplus Y$.

(25) $A = 0$, $B = C_1$, $W = B$, $X = C_2$, $Y = B \oplus X$ and $Z = W$.

(26) $A = 0$, $B = 0$, $W = C_1$, $X = C_2$, $Y = X$ and $Z = W \oplus Y$.

(27) $A = 0$, $B = C_1$, $W = B$, $X = C_2$, $Y = B \oplus X$ and $Z = W \oplus Y$.

(28) $A = 0$, $B = C_1$, $W = B$, $X = C_2$, $Y = B \oplus X$ and $Z = Y$.

(29) $A = 0$, $B = 0$, $W = C_1$, $X = 0$, $Y = C_2$ and $Z = W \oplus Y$.

(30) $A = 0$, $B = C_1$, $W = B$, $X = C_2$, $Y = B \oplus X$ and $Z = 0$.

(31) $A = 0$, $B = 0$, $W = 0$, $X = 0$, $Y = 0$ and $Z = C_1$.

(32) $A = 0$, $B = 0$, $W = 0$, $X = 0$, $Y = C_1$ and $Z = 0$.

(33) $A = 0$, $B = 0$, $W = 0$, $X = C_1$, $Y = 0$ and $Z = 0$.

(34) $A = 0$, $B = 0$, $W = C_1$, $X = 0$, $Y = 0$ and $Z = 0$.

(35) $A = 0$, $B = 0$, $W = 0$, $X = 0$, $Y = C_1$ and $Z = Y$.

(36) $A = 0$, $B = 0$, $W = 0$, $X = C_1$, $Y = X$ and $Z = 0$.

(37) $A = 0$, $B = 0$, $W = C_1$, $X = 0$, $Y = 0$ and $Z = W$.

(38) $A = 0$, $B = C_1$, $W = B$, $X = 0$, $Y = B$ and $Z = 0$.

(39) $A = 0$, $B = 0$, $W = 0$, $X = C_1$, $Y = X$ and $Z = Y$.

(40) $A = 0$, $B = C_1$, $W = B$, $X = 0$, $Y = B$ and $Z = Y$.

These 40 extremal rays are also extremal rays of the outer approximation to the entropy cone of causal structure 4 by means of Shannon and independence constraints. This outer approximation has only one additional extremal ray,

$$(S1) \quad 2\ 2\ 3\ 2\ 4\ 4\ 3\ 4\ 3\ 4\ 5\ 4\ 5\ 5\ 5.$$

[1] Note that this strategy recovers double the entropy vector listed above.

## Causal Structure 5

We provide the vertex description of an inner approximation to the marginal entropy cone of Causal Structure 5 in terms of one vector on each extremal ray, with components ordered as

$$(H(W),\ H(X),\ H(Y),\ H(Z),\ H(WX),\ H(WY),\ H(WZ),\ H(XY),\ H(XZ),\ H(YZ),\ H(WXY),\ H(WXZ),\ H(WYZ),\ H(XYZ),\ H(WXYZ))\ .$$

(1) 2 2 2 3 3 4 4 4 4 5 5 5 5 5 5
(2) 2 2 2 3 3 4 4 3 3 4 4 4 4 4 4
(3) 2 2 2 2 3 4 4 3 3 4 4 4 4 4 4
(4) 2 2 1 3 4 3 4 3 4 4 5 5 5 5 5
(5) 2 2 1 2 4 3 3 3 4 3 5 5 4 5 5
(6) 2 2 1 2 3 3 3 3 3 3 4 4 4 4 4
(7) 1 1 2 2 2 3 3 3 3 4 4 4 4 4 4
(8) 1 1 2 2 2 3 3 2 2 3 3 3 3 3 3
(9) 1 2 1 2 2 2 2 3 3 3 3 3 3 3 3
(10) 1 2 1 2 2 2 2 2 2 2 2 2 2 2 2
(11) 1 1 1 3 2 2 3 2 3 3 3 3 3 3 3
(12) 1 1 1 2 2 2 3 2 3 3 3 3 3 3 3
(13) 1 1 1 2 2 2 2 2 3 3 3 3 3 3 3
(14) 1 1 1 2 2 2 3 2 2 3 3 3 3 3 3
(15) 1 1 2 1 2 3 2 2 2 3 3 3 3 3 3
(16) 1 1 1 2 2 2 2 2 2 3 3 2 3 3 3
(17) 1 1 1 2 2 2 2 2 3 2 3 3 2 3 3
(18) 1 2 1 1 2 2 2 2 2 2 2 2 2 2 2
(19) 1 1 1 1 2 2 2 2 2 2 3 3 3 3 3
(20) 2 2 2 2 3 4 3 3 3 4 4 4 4 4 4
(21) 1 1 1 1 2 2 2 2 2 2 3 3 2 3 3
(22) 1 1 1 2 1 2 2 2 2 2 2 2 2 2 2
(23) 1 1 1 2 2 2 2 1 2 2 2 2 2 2 2
(24) 1 2 1 1 2 2 1 2 2 2 2 2 2 2 2
(25) 1 1 1 1 2 2 1 2 2 2 3 2 2 3 3
(26) 1 1 1 1 1 2 2 2 2 2 2 2 2 2 2
(27) 1 1 1 1 2 2 2 1 2 2 2 2 2 2 2
(28) 0 1 1 1 1 1 1 2 2 2 2 2 2 2 2
(29) 1 1 0 1 2 1 2 1 2 1 2 2 2 2 2
(30) 0 0 0 1 0 0 1 0 1 1 0 1 1 1 1
(31) 0 0 1 0 0 1 0 1 0 1 1 0 1 1 1
(32) 0 1 0 0 1 0 0 1 1 0 1 1 0 1 1
(33) 1 0 0 0 1 1 1 0 0 0 1 1 1 0 1
(34) 1 1 1 1 1 2 1 2 1 2 2 1 2 2 2
(35) 1 1 1 1 2 2 1 1 2 2 2 2 2 2 2
(36) 0 0 1 1 0 1 1 1 1 1 1 1 1 1 1
(37) 0 1 0 1 1 0 1 1 1 1 1 1 1 1 1
(38) 0 1 1 0 1 1 0 1 1 1 1 1 1 1 1
(39) 1 1 0 0 1 1 1 1 1 0 1 1 1 1 1
(40) 0 1 1 1 1 1 1 1 1 1 1 1 1 1 1
(41) 1 1 1 0 1 1 1 1 1 1 1 1 1 1 1
(42) 1 1 1 1 1 1 1 1 1 1 1 1 1 1 1

In the following we list strategies to recover entropy vectors on all of the above rays. $C_1$, $C_2$, $C_3$, $C_4$ and $C_5$ are uniform bits, $\oplus$ denotes addition modulus 2.

(1) $A = (A_1,\ A_2) = (C_1,\ C_2)$, $B = C_3$, $W = (W_1,\ W_2) = (C_4,\ C_5)$, $X = (X_1,\ X_2) = (W_1,\ B \oplus W_2)$, $Y = (Y_1,\ Y_2) = (A_1 \oplus X_1,\ A_2 \oplus X_2)$ and $Z = (A_1 \oplus Y_1,\ B \oplus Y_2,\ A_1 \oplus A_2 \oplus B)$.

(2) $A = C_1$, $B = C_2$, $W = (W_1,\ W_2) = (C_3,\ C_4)$, $X = (X_1,\ X_2) = (B \oplus W_1,\ B \oplus W_2)$, $Y = (Y_1,\ Y_2) = (X_1,\ A \oplus X_2)$ and $Z = (A \oplus B \oplus Y_1,\ A \oplus Y_2,\ A \oplus B)$.

(3) $A = C_1$, $B = C_2$, $W = (W_1,\ W_2) = (C_3,\ C_4)$, $X = (X_1,\ X_2) = (B \oplus W_1,\ B \oplus W_2)$, $Y = (Y_1,\ Y_2) = (X_1,\ A \oplus X_2)$ and $Z = (A \oplus B \oplus Y_1,\ A \oplus Y_2)$.

(4) $A = C_1$, $B = (B_1,\ B_2) = (C_2,\ C_3)$, $W = (W_1,\ W_2) = (C_4,\ C_5)$, $X = (X_1,\ X_2) = (B_1 \oplus W_1,\ B_2 \oplus W_2)$, $Y = A \oplus X_1$ and $Z = (A \oplus B_1 \oplus Y,\ A \oplus Y,\ A \oplus B_2)$.

(5) $A = C_1$, $B = (B_1,\ B_2) = (C_2,\ C_3)$, $W = (W_1,\ W_2) = (C_4,\ C_5)$, $X = (X_1,\ X_2) = (B_1 \oplus W_1,\ B_2 \oplus W_2)$, $Y = A \oplus X_1$ and $Z = (A \oplus B_1 \oplus Y,\ B_1 \oplus B_2 \oplus Y)$.

(6) $A = C_1$, $B = C_2$, $W = (W_1,\ W_2) = (C_3,\ C_4)$, $X = (X_1,\ X_2) = (B \oplus W_1,\ W_2)$, $Y = A \oplus X_2$ and $Z = (A \oplus Y,\ A \oplus B)$.

(7) $A = (A_1,\ A_2) = (C_1,\ C_2)$, $B = C_3$, $W = C_4$, $X = B \oplus W$, $Y = (Y_1,\ Y_2) = (A_1 \oplus X,\ A_2)$ and $Z = (A_1 \oplus A_2,\ A_1 \oplus B)$.

(8) $A = C_1$, $B = C_2$, $W = C_3$, $X = B \oplus W$, $Y = (Y_1,\ Y_2) = (X,\ A)$ and $Z = (Y_1,\ A \oplus B \oplus Y_1)$.

(9) $A = C_1$, $B = C_2$, $W = C_3$, $X = (X_1,\ X_2) = (W,\ B)$, $Y = A \oplus X_1 \oplus X_2$ and $Z = (A \oplus B \oplus Y,\ B \oplus Y)$.

(10) $A = 0$, $B = C_1$, $W = C_2$, $X = (X_1,\ X_2) = (B,\ W)$, $Y = X_1 \oplus X_2$ and $Z = (B \oplus Y,\ B)$.

(11) $A = C_1$, $B = C_2$, $W = C_3$, $X = B \oplus W$, $Y = A \oplus X$ and $Z = (B,\ A,\ A \oplus Y)$.

(12) $A = C_1$, $B = C_2$, $W = C_3$, $X = B \oplus W$, $Y = A \oplus X$ and $Z = (B,\ A)$.

(13) $A = C_1$, $B = C_2$, $W = C_3$, $X = B \oplus W$, $Y = A \oplus X$ and $Z = (A \oplus B \oplus Y,\ A)$.

(14) $A = C_1$, $B = C_2$, $W = C_3$, $X = B \oplus W$, $Y = A \oplus X$ and $Z = (A \oplus Y,\ A \oplus B)$.

(15) $A = C_1$, $B = C_2$, $W = C_3$, $X = B \oplus W$, $Y = (Y_1,\ Y_2) = (A,\ X)$ and $Z = A \oplus B$.

(16) $A = C_1$, $B = C_2$, $W = C_3$, $X = B \oplus W$, $Y = A \oplus X$ and $Z = (A \oplus B \oplus Y,\ A \oplus Y)$.

(17) $A = C_1$, $B = C_2$, $W = C_3$, $X = B \oplus W$, $Y = A \oplus X$ and $Z = (Y,\ A \oplus B \oplus Y)$.

(18) $A = 0$, $B = C_1$, $W = C_2$, $X = (X_1,\ X_2) = (W,\ B)$, $Y = X_1 \oplus X_2$ and $Z = B$.

(19) $A = C_1$, $B = C_2$, $W = C_3$, $X = B \oplus W$, $Y = A \oplus X$ and $Z = B \oplus Y$.

(20) $A = C_1$, $B = C_2$, $W = (W_1,\ W_2) = (C_3,\ C_4)$, $X = (X_1,\ X_2) = (B \oplus W_1,\ W_2)$, $Y = (Y_1,\ Y_2) = (X_1,\ A \oplus X_2)$ and $Z = (A \oplus B \oplus Y_1,\ A \oplus Y_2)$.

(21) $A = C_1$, $B = C_2$, $W = C_3$, $X = B \oplus W$, $Y = A \oplus X$ and $Z = A \oplus B$.

(22) $A = C_1$, $B = 0$, $W = C_2$, $X = W$, $Y = A \oplus X$ and $Z = (A,\ Y)$.

(23) $A = 0$, $B = C_1$, $W = C_2$, $X = B \oplus W$, $Y = X$ and $Z = (B,\ Y)$.

(24) $A = 0$, $B = C_1$, $W = C_2$, $X = (X_1,\ X_2) = (W,\ B)$, $Y = X_1 \oplus X_2$ and $Z = B \oplus Y$.

(25) $A = C_1$, $B = C_2$, $W = C_3$, $X = B \oplus W$, $Y = A \oplus X$ and $Z = A \oplus B \oplus Y$.

(26) $A = C_1$, $B = 0$, $W = C_2$, $X = W$, $Y = A \oplus X$ and $Z = A$.

(27) $A = 0$, $B = C_1$, $W = C_3$, $X = B \oplus W$, $Y = X$ and $Z = B$.

(28) $A = C_1$, $B = C_2$, $W = 0$, $X = B$, $Y = A \oplus X$ and $Z = A$.

(29) $A = 0$, $B = C_1$, $W = C_2$, $X = B \oplus W$, $Y = 0$ and $Z = B$.

(30) $A = 0$, $B = 0$, $W = 0$, $X = 0$, $Y = 0$ and $Z = C_1$.

(31) $A = 0$, $B = 0$, $W = 0$, $X = 0$, $Y = C_1$ and $Z = 0$.

(32) $A = 0$, $B = 0$, $W = 0$, $X = C_1$, $Y = 0$ and $Z = 0$.

(33) $A = 0$, $B = 0$, $W = C_1$, $X = 0$, $Y = 0$ and $Z = 0$.

(34) $A = C_1$, $B = 0$, $W = C_2$, $X = W$, $Y = A \oplus X$ and $Z = A \oplus Y$.

(35) $A = 0$, $B = C_1$, $W = C_2$, $X = B \oplus W$, $Y = X$ and $Z = B \oplus Y$.

(36) $A = 0$, $B = 0$, $W = 0$, $X = 0$, $Y = C_1$ and $Z = Y$.

(37) $A = 0$, $B = C_1$, $W = 0$, $X = B$, $Y = 0$ and $Z = B$.

(38) $A = 0$, $B = 0$, $W = 0$, $X = C_1$, $Y = X$ and $Z = 0$.

(39) $A = 0$, $B = 0$, $W = C_1$, $X = W$, $Y = 0$ and $Z = 0$.

(40) $A = 0$, $B = 0$, $W = 0$, $X = C_1$, $Y = X$ and $Z = Y$.

(41) $A = 0$, $B = 0$, $W = C_1$, $X = W$, $Y = X$ and $Z = 0$.

(42) $A = 0$, $B = 0$, $W = C_1$, $X = W$, $Y = X$ and $Z = Y$.

These 42 extremal rays are also extremal rays of the outer approximation to the entropy cone of causal structure 5 by means of Shannon and independence constraints. This outer approximation has 7 additional extremal rays,

| | |
|---|---|
| $(S1)$ | 3 3 2 3 5 5 4 4 5 4 6 6 5 6 6 |
| $(S2)$ | 3 3 2 3 5 4 4 4 6 4 6 6 5 6 6 |
| $(S3)$ | 3 3 2 3 4 5 4 4 4 4 5 5 5 5 5 |
| $(S4)$ | 2 2 2 2 3 3 3 3 3 4 4 4 4 4 4 |
| $(S5)$ | 2 2 2 2 3 3 3 3 4 3 4 4 4 4 4 |
| $(S6)$ | 2 2 2 2 3 3 4 3 3 3 4 4 4 4 4 |
| $(S7)$ | 2 2 2 2 3 4 3 3 3 3 4 4 4 4 4 |

## Causal Structure 6

We provide the vertex description of an inner approximation to the marginal entropy cone of Causal Structure 6 in terms of one vector on each extremal ray, with components ordered as

$$(H(W),\ H(X),\ H(Y),\ H(Z),\ H(WX),\ H(WY),\ H(WZ),\ H(XY),\ H(XZ),\ H(YZ),\ H(WXY),\ H(WXZ),\ H(WYZ),\ H(XYZ),\ H(WXYZ))\ .$$

| | |
|---|---|
| (1) | 2 3 2 2 4 4 3 5 4 4 5 5 4 5 5 |
| (2) | 2 3 2 2 4 3 3 5 5 4 5 5 4 5 5 |
| (3) | 2 3 1 2 4 3 3 4 4 3 5 5 4 5 5 |
| (4) | 2 2 1 2 4 3 3 3 4 3 5 5 4 5 5 |
| (5) | 2 2 2 1 3 3 2 4 3 3 4 3 3 4 4 |
| (6) | 1 3 1 2 3 2 2 4 4 3 4 4 3 4 4 |
| (7) | 2 1 2 1 3 4 3 3 2 3 4 4 4 4 4 |
| (8) | 1 2 1 2 3 2 3 3 4 3 4 4 3 4 4 |
| (9) | 1 2 1 2 3 2 2 3 4 3 4 4 3 4 4 |
| (10) | 1 2 2 1 2 3 2 3 3 3 3 3 3 3 3 |
| (11) | 2 1 1 2 3 3 3 2 3 2 3 3 3 3 3 |
| (12) | 1 1 2 2 2 3 3 2 2 3 3 3 3 3 3 |
| (13) | 2 2 1 1 3 3 2 3 2 2 3 3 3 3 3 |
| (14) | 1 2 1 2 2 2 2 3 3 2 3 3 2 3 3 |
| (15) | 1 2 1 2 2 2 2 2 2 2 2 2 2 2 2 |
| (16) | 1 1 2 1 2 3 2 3 2 3 3 3 3 3 3 |
| (17) | 1 2 1 1 3 2 2 3 3 2 3 3 3 3 3 |
| (18) | 2 1 1 1 3 3 3 2 2 2 3 3 3 3 3 |
| (19) | 1 1 2 1 2 3 2 2 2 3 3 3 3 3 3 |
| (20) | 2 1 1 1 3 3 2 2 2 2 3 3 3 3 3 |
| (21) | 1 2 1 1 2 2 2 3 3 2 3 3 2 3 3 |
| (22) | 1 1 1 2 2 2 2 2 3 2 3 3 2 3 3 |
| (23) | 1 1 1 2 2 2 2 2 2 2 2 2 2 2 2 |
| (24) | 1 1 2 1 2 2 2 2 2 2 2 2 2 2 2 |
| (25) | 1 2 1 1 2 2 2 2 2 2 2 2 2 2 2 |
| (26) | 1 1 1 1 2 2 2 2 2 2 3 3 3 3 3 |
| (27) | 1 1 1 1 2 2 2 2 2 2 3 3 2 3 3 |
| (28) | 1 2 1 1 2 2 1 3 2 2 3 2 2 3 3 |
| (29) | 1 1 1 1 2 2 2 2 2 2 2 2 2 2 2 |
| (30) | 1 1 1 2 2 2 2 1 2 2 2 2 2 2 2 |
| (31) | 1 2 1 1 2 2 1 2 2 2 2 2 2 2 2 |
| (32) | 1 1 1 1 2 2 1 2 2 2 3 2 2 3 3 |
| (33) | 1 1 1 1 2 1 2 2 2 2 2 2 2 2 2 |
| (34) | 1 1 1 1 2 2 1 2 2 2 2 2 2 2 2 |
| (35) | 1 1 1 1 2 2 2 1 2 2 2 2 2 2 2 |
| (36) | 1 1 1 1 2 2 2 2 1 2 2 2 2 2 2 |
| (37) | 1 1 1 1 2 2 2 2 2 1 2 2 2 2 2 |
| (38) | 0 1 1 1 1 1 1 2 2 2 2 2 2 2 2 |
| (39) | 1 1 0 1 2 1 2 1 2 1 2 2 2 2 2 |
| (40) | 1 1 1 0 2 2 1 2 1 1 2 2 2 2 2 |
| (41) | 1 1 1 1 2 2 1 1 2 2 2 2 2 2 2 |
| (42) | 0 0 0 1 0 0 1 0 1 1 0 1 1 1 1 |
| (43) | 0 0 1 0 0 1 0 1 0 1 1 0 1 1 1 |
| (44) | 0 1 0 0 1 0 0 1 1 0 1 1 0 1 1 |
| (45) | 1 0 0 0 1 1 1 0 0 0 1 1 1 0 1 |
| (46) | 0 0 1 1 0 1 1 1 1 1 1 1 1 1 1 |
| (47) | 0 1 0 1 1 0 1 1 1 1 1 1 1 1 1 |
| (48) | 0 1 1 0 1 1 0 1 1 1 1 1 1 1 1 |
| (49) | 1 0 1 0 1 1 1 1 0 1 1 1 1 1 1 |
| (50) | 1 1 0 0 1 1 1 1 1 0 1 1 1 1 1 |
| (51) | 0 1 1 1 1 1 1 1 1 1 1 1 1 1 1 |
| (52) | 1 0 1 1 1 1 1 1 1 1 1 1 1 1 1 |
| (53) | 1 1 1 0 1 1 1 1 1 1 1 1 1 1 1 |
| (54) | 1 1 1 1 1 1 1 1 1 1 1 1 1 1 1 |

In the following we list strategies to recover entropy vectors on all of the above rays. $C_1$, $C_2$, $C_3$, $C_4$ and $C_5$ are uniform bits, $\oplus$ denotes addition modulus 2.

(1) $W = (W_1,\ W_2) = (C_1,\ C_2)$, $B = (B_1,\ B_2) = (C_3,\ C_4)$, $A = (A_1,\ A_2,\ A_3) = (W_1,\ W_2,\ C_5)$, $X = (X_1,\ X_2,\ X_3) = (A_1,\ A_1 \oplus A_3 \oplus B_2,\ A_3 \oplus B_1)$, $Y = (Y_1,\ Y_2) = (A_3 \oplus X_1 \oplus X_3,\ A_1 \oplus A_2 \oplus A_3 \oplus X_2)$ and $Z = (B_1 \oplus Y_1,\ B_2)$.

(2) $W = (W_1,\ W_2) = (C_1,\ C_2)$, $B = (B_1,\ B_2) = (C_3,\ C_4)$, $A = (A_1,\ A_2,\ A_3) = (W_1,\ W_2,\ C_5)$, $X = (X_1,\ X_2,\ X_3) = (A_1,\ A_2 \oplus A_3 \oplus B_1,\ A_2 \oplus A_3 \oplus B_2)$, $Y = (Y_1,\ Y_2) = (A_1 \oplus A_2,\ A_1 \oplus A_2 \oplus A_3 \oplus X_2)$ and $Z = (B_1 \oplus Y_1 \oplus Y_2,\ B_2)$.

(3) $W = (W_1,\ W_2) = (C_1,\ C_2)$, $B = (B_1,\ B_2) = (C_3,\ C_4)$, $A = (A_1,\ A_2,\ A_3) = (W_1,\ W_2,\ C_5)$, $X = (X_1,\ X_2,\ X_3) = (A_1 \oplus A_2,\ A_2 \oplus A_3 \oplus B_1,\ A_3 \oplus B_2)$, $Y = A_3 \oplus X_1 \oplus X_3$ and $Z = (B_2 \oplus Y,\ B_1)$.

(4) $W = (W_1,\ W_2) = (C_1,\ C_2)$, $B = (B_1,\ B_2) = (C_3,\ C_4)$, $A = (A_1,\ A_2,\ A_3) = (W_1,\ W_2,\ C_5)$, $X = (X_1,\ X_2) = (A_1 \oplus A_3 \oplus B_1,\ A_2 \oplus B_2)$, $Y = A_3 \oplus X_1$ and $Z = (B_1 \oplus Y,\ B_1 \oplus B_2)$.

(5) $W = (W_1,\ W_2) = (C_1,\ C_2)$, $B = C_3$, $A = (A_1,\ A_2,\ A_3) = (W_1,\ W_2,\ C_4)$, $X = (X_1,\ X_2) = (A_1,\ A_2 \oplus A_3 \oplus B)$, $Y = (Y_1,\ Y_2) = (A_1 \oplus A_2,\ A_3 \oplus X_2)$ and $Z = Y_2 \oplus B$.

(6) $W = C_1$, $B = (B_1,\ B_2) = (C_2,\ C_3)$, $A = (A_1,\ A_2) = (W,\ C_4)$, $X = (X_1,\ X_2,\ X_3) = (A_1,\ B_1,\ A_2 \oplus B_2)$, $Y = A_1 \oplus A_2 \oplus X_2 \oplus X_3$ and $Z = (B_1 \oplus B_2 \oplus Y,\ B_2)$.

(7) $W = (W_1,\ W_2) = (C_1,\ C_2)$, $B = C_3$, $A = (A_1,\ A_2,\ A_3) = (W_1,\ W_2,\ C_4)$, $X = A_3 \oplus B$, $Y = (Y_1,\ Y_2) = (A_1 \oplus A_3 \oplus X,\ A_2 \oplus X)$ and $Z = B$.

(8) $W = C_1$, $B = (B_1,\ B_2) = (C_2,\ C_3)$, $A = (A_1,\ A_2) = (W,\ C_4)$, $X = (X_1,\ X_2) = (B_1,\ A_2 \oplus B_2)$, $Y = A_1 \oplus A_2 \oplus X_2$ and $Z = (B_1 \oplus Y,\ B_2)$.

(9) $W = C_1$, $B = (B_1,\ B_2) = (C_2,\ C_3)$, $A = (A_1,\ A_2) = (W,\ C_4)$, $X = (X_1,\ X_2) = (A_1 \oplus B_1,\ A_2 \oplus B_2)$, $Y = A_1 \oplus A_2 \oplus X_2$ and $Z = (B_2 \oplus Y,\ B_1 \oplus B_2)$.

(10) $W = C_1$, $B = C_2$, $A = (A_1,\ A_2) = (W,\ C_3)$, $X = (X_1,\ X_2) = (A_2 \oplus B,\ A_1)$, $Y = (Y_1,\ Y_2) = (X_1,\ A_1 \oplus A_2)$ and $Z = B$.

(11) $W = (W_1,\ W_2) = (C_1,\ C_2)$, $B = C_3$, $A = (A_1,\ A_2) = (W_1,\ W_2)$, $X = A_2 \oplus B$, $Y = A_1 \oplus X$ and $Z = (B \oplus Y, B)$.

(12) $W = C_1$, $B = C_2$, $A = (A_1,\ A_2) = (W,\ C_3)$, $X = A_1 \oplus B$, $Y = (Y_1,\ Y_2) = (X,\ A_2)$ and $Z = (Y_1,\ B \oplus Y_2)$.

(13) $W = (W_1,\ W_2) = (C_1,\ C_2)$, $B = C_3$, $A = (A_1,\ A_2) = (W_1,\ W_2)$, $X = (X_1,\ X_2) = (A_1, A_2 \oplus B)$, $Y = A_1 \oplus A_2 \oplus X_2$ and $Z = B \oplus Y$.

(14) $W = C_1$, $B = C_2$, $A = (A_1,\ A_2) = (W,\ C_3)$, $X = (X_1,\ X_2) = (A_1, A_2 \oplus B)$, $Y = A_2 \oplus X_1 \oplus X_2$ and $Z = (B \oplus Y,\ B)$.

(15) $W = C_1$, $B = C_2$, $A = W$, $X = (X_1,\ X_2) = (A, B)$, $Y = X_1 \oplus X_2$ and $Z = (B \oplus Y,\ B)$.

(16) $W = C_1$, $B = C_2$, $A = (W,\ C_3)$, $X = B$, $Y = (X \oplus A_2,\ A_1 \oplus A_2)$ and $Z = B \oplus Y$.

(17) $W = C_1$, $B = C_2$, $A = (W,\ C_3)$, $X = (X_1,\ X_2) = (A_1 \oplus B,\ A_2)$, $Y = A_1 \oplus A_2$ and $Z = B$.

(18) $W = (W_1,\ W_2) = (C_1,\ C_2)$, $B = C_3$, $A = (A_1,\ A_2) = (W_1,\ W_2)$, $X = A_1 \oplus B$, $Y = A_1 \oplus A_2 \oplus X$ and $Z = B$.

(19) $W = C_1$, $B = C_2$, $A = (A_1,\ A_2) = (W,\ C_3)$, $X = A_1 \oplus B$, $Y = (Y_1,\ Y_2) = (X,\ A_2)$ and $Z = B \oplus Y_1 \oplus Y_2$.

(20) $W = (W_1,\ W_2) = (C_1,\ C_2)$, $B = C_3$, $A = (A_1,\ A_2) = (W_1,\ W_2)$, $X = A_1 \oplus A_2 \oplus B$, $Y = A_2 \oplus X$ and $Z = B \oplus Y$.

(21) $W = C_1$, $B = C_2$, $A = (A_1,\ A_2) = (W,\ C_3)$, $X = (X_1,\ X_2) = (A_2 \oplus B,\ A_1)$, $Y = A_1 \oplus A_2 \oplus X_1$ and $Z = B$.

(22) $W = C_1$, $B = C_2$, $A = (A_1,\ A_2) = (W,\ C_3)$, $X = A_2 \oplus B$, $Y = A_1 \oplus A_2 \oplus X$ and $Z = (B \oplus Y,\ B)$.

(23) $W = C_1$, $B = C_2$, $A = W$, $X = B$, $Y = A \oplus X$ and $Z = (B \oplus Y,\ B)$.

(24) $W = C_1$, $B = C_2$, $A = W$, $X = A \oplus B$, $Y = (Y_1,\ Y_2) = (A,\ A \oplus X)$ and $Z = B$.

(25) $W = C_1$, $B = C_2$, $A = W$, $X = (X_1,\ X_2) = (A,\ B)$, $Y = X_1 \oplus X_2$ and $Z = B$.

(26) $W = C_1$, $B = C_2$, $A = W$, $X = A \oplus B$, $Y = X \oplus C_3$ and $Z = B \oplus Y$.

(27) $W = C_1$, $B = C_2$, $A = (A_1,\ A_2) = (W,\ C_3)$, $X = A_1 \oplus A_2 \oplus B$, $Y = X \oplus A_2$ and $Z = B$.

(28) $W = C_1$, $B = C_2$, $A = (A_1,\ A_2) = (W,\ C_3)$, $X = (X_1,\ X_2) = (A_1,\ A_2 \oplus B)$, $Y = A_1 \oplus A_2 \oplus X_2$ and $Z = B \oplus Y$.

(29) $W = (W_1,\ W_2) = (C_1,\ C_2)$, $B = (B_1,\ B_2) = (C_3,\ C_4)$, $A = (A_1,\ A_2) = (W_1,\ W_2)$, $X = (X_1,\ X_2) = (A_1 \oplus B_1,\ A_2 \oplus B_2)$, $Y = (Y_1,\ Y_2) = (A_1 \oplus A_2 \oplus X_1, A_1 \oplus X_2)$ and $Z = (B_1, B_2)$. [2]

(30) $W = C_1$, $B = C_2$, $A = W$, $X = A \oplus B$, $Y = X$ and $Z = (B,\ Y)$.

(31) $W = C_1$, $B = C_2$, $A = W$, $X = (X_1,\ X_2) = (B,\ A)$, $Y = A \oplus X_1$ and $Z = B \oplus Y$.

(32) $W = C_1$, $B = C_2$, $A = (A_1,\ A_2) = (W,\ C_3)$, $X = A_2 \oplus B$, $Y = A_1 \oplus A_2 \oplus X$ and $Z = B \oplus Y$.

(33) $W = C_1$, $B = C_2$, $A = W$, $X = A \oplus B$, $Y = A$ and $Z = B$.

(34) $W = C_1$, $B = C_2$, $A = W$, $X = B$, $Y = A \oplus X$ and $Z = B \oplus Y$.

(35) $W = C_1$, $B = C_2$, $A = W$, $X = A \oplus B$, $Y = X$ and $Z = B$.

(36) $W = C_1$, $B = C_2$, $A = W$, $X = B$, $Y = A \oplus X$ and $Z = B$.

(37) $W = C_1$, $B = C_2$, $A = W$, $X = A \oplus B$, $Y = A \oplus X$ and $Z = Y$.

(38) $W = 0$, $B = C_1$, $A = C_2$, $X = A \oplus B$, $Y = A$ and $Z = B$.

(39) $W = C_1$, $B = C_2$, $A = W$, $X = A \oplus B$, $Y = 0$ and $Z = B$.

(40) $W = C_1$, $B = C_2$, $A = W$, $X = B$, $Y = A \oplus X$ and $Z = 0$.

(41) $W = C_1$, $B = C_2$, $A = W$, $X = A \oplus B$, $Y = X$ and $Z = B \oplus Y$.

(42) $W = 0$, $B = 0$, $A = 0$, $X = 0$, $Y = 0$ and $Z = C_1$.

(43) $W = 0$, $B = 0$, $A = 0$, $X = 0$, $Y = C_1$ and $Z = 0$.

(44) $W = 0$, $B = 0$, $A = 0$, $X = C_1$, $Y = 0$ and $Z = 0$.

(45) $W = C_1$, $B = 0$, $A = 0$, $X = 0$, $Y = 0$ and $Z = 0$.

(46) $W = 0$, $B = 0$, $A = 0$, $X = 0$, $Y = C_1$ and $Z = Y$.

(47) $W = 0$, $B = C_1$, $A = 0$, $X = B$, $Y = 0$ and $Z = B$.

(48) $W = 0$, $B = 0$, $A = 0$, $X = C_1$, $Y = X$ and $Z = 0$.

(49) $W = C_1$, $B = 0$, $A = W$, $X = 0$, $Y = A$ and $Z = 0$.

(50) $W = C_1$, $B = 0$, $A = W$, $X = A$, $Y = 0$ and $Z = 0$.

(51) $W = 0$, $B = 0$, $A = 0$, $X = C_1$, $Y = X$ and $Z = Y$.

(52) $W = C_1$, $B = 0$, $A = W$, $X = 0$, $Y = A$ and $Z = Y$.

(53) $W = C_1$, $B = 0$, $A = W$, $X = A$, $Y = X$ and $Z = 0$.

(54) $W = C_1$, $B = 0$, $A = W$, $X = A$, $Y = X$ and $Z = Y$.

These 54 extremal rays are also extremal rays of the outer approximation to the entropy cone of causal structure 6 by means of Shannon and independence constraints. This outer approximation has 12 additional extremal rays,

| | | | |
|---|---|---|---|
| $(S1)$ | 3 4 2 3 5 5 4 5 5 4 6 6 5 6 6 | $(S7)$ | 2 3 2 2 4 3 3 4 4 4 5 5 4 5 5 |
| $(S2)$ | 3 4 2 3 5 4 4 6 5 4 6 6 5 6 6 | $(S8)$ | 2 2 2 2 3 3 3 3 4 3 4 4 4 4 4 |
| $(S3)$ | 3 3 2 3 5 5 4 4 5 4 6 6 5 6 6 | $(S9)$ | 2 2 2 2 3 3 3 4 3 3 4 4 4 4 4 |
| $(S4)$ | 3 3 2 3 5 4 4 4 6 4 6 6 5 6 6 | $(S10)$ | 2 2 2 2 3 3 4 3 3 3 4 4 4 4 4 |
| $(S5)$ | 2 3 3 2 4 4 3 4 4 5 5 5 5 5 5 | $(S11)$ | 2 2 2 2 3 4 3 3 3 3 4 4 4 4 4 |
| $(S6)$ | 3 2 2 3 5 4 4 3 4 4 5 5 5 5 5 | $(S12)$ | 2 2 2 2 4 3 3 3 3 3 4 4 4 4 4 |

# References

[1] Henson, J., Lal, R. & Pusey, M. F. Theory-independent limits on correlations from generalized Bayesian networks. *New Journal of Physics* **16**, 113043 (2014).

[2] Note that this strategy recovers double the entropy vector listed above.
